# Supplementary material for: Quartic graphs which are Bakry-\'Emery curvature sharp
Source: arXiv:1902.10665 ancillary file (2019-02-27)
Supplement: Supplementary file 1 [file classification.pdf]

# Incomplete 2-Balls for Quartic Graphs

Francis Gurr and Leyna Watson May

## Abstract

This document contains the 365 incomplete 2-balls, separated by structure of the 1-ball. Additionally, it contains the 22 2-balls with infinity curvature sharp centres. This Latex document was generated by a Python program with the help of a curvature calculator written by David Cushing and George Stagg, see [CKLLS17].

## Representation of 2-balls

The (incomplete) 2-balls of quartic graphs listed in this article are represented in the following way. We fix a vertex  $v_0$  and  $S_1(v_0) = \{v_1, v_2, v_3, v_4\}$  (since in a quartic graph,  $v_0$  has four neighbors). The vertices of the 2-sphere are labeled as follows:  $S_2(v_0) = \{v_5, v_6, \dots, v_m\}$ . Then a 2-ball  $B_2(v_0)$  centered at  $v_0$  is represented by a list of 3 lists:  $B_2(v_0) = [list_1, list_2, list_3]$ . The first list determines the  $S_1$  structure (i.e., how the vertices in  $S_1$  are connected to each other) by  $list_1 = [a_{12}, a_{13}, a_{14}, a_{23}, a_{24}, a_{34}]$  where each  $a_{ij} \in \{0, 1\}$  is a Boolean indicator whether vertices  $v_i$  and  $v_j$  are adjacent or not. The second list  $list_2 = [a_5, a_6, \dots, a_m]$  describes the  $S_1$ - $S_2$  structure (i.e., which vertices in  $S_2$  are adjacent to vertices in  $S_1$ ). For instance,  $a_5 = [1, 2, 3]$  means that the vertex  $v_5$  is adjacent to  $v_1, v_2, v_3$  but not to  $v_4$ . Lastly, the list  $list_3$  describes the  $S_2$  structure (i.e., how the vertices in  $S_2$  are connected to each other). For example,  $list_3 = [[5, 7], [5, 8], [6, 8]]$  means that  $v_5 \sim v_7$ ,  $v_5 \sim v_8$ , and  $v_6 \sim v_8$ . However, the computation of Bakry-Émery curvature only requires the information of incomplete 2-balls where no spherical edge of  $S_2(v_0)$  is present, in which case  $list_3 = []$ .

The 11 1-ball structures and relevant properties are summarised in the following table:

| Index | 1-Ball             | $S_1$ -out regular | Bakry-Émery curvature bound, $\kappa_\infty$ | Total number of 2-Balls |
|-------|--------------------|--------------------|----------------------------------------------|-------------------------|
| 1     | [0, 0, 0, 0, 0, 0] | True               | 2.000                                        | 93                      |
| 2     | [1, 0, 0, 0, 0, 0] | False              | 2.250                                        | 120                     |
| 3     | [1, 0, 0, 0, 0, 1] | True               | 2.500                                        | 40                      |
| 4     | [1, 1, 0, 0, 0, 0] | False              | 2.500                                        | 55                      |
| 5     | [1, 1, 1, 0, 0, 0] | False              | 2.750                                        | 8                       |
| 6     | [1, 1, 0, 1, 0, 0] | False              | 2.750                                        | 10                      |
| 7     | [1, 1, 0, 0, 1, 0] | False              | 2.750                                        | 24                      |
| 8     | [1, 1, 0, 0, 1, 1] | True               | 3.000                                        | 7                       |
| 9     | [1, 1, 1, 1, 0, 0] | False              | 3.000                                        | 5                       |
| 10    | [1, 1, 1, 1, 1, 0] | False              | 3.250                                        | 2                       |
| 11    | [1, 1, 1, 1, 1, 1] | True               | 3.500                                        | 1                       |

1  $list_1 = [0, 0, 0, 0, 0, 0]$

$S_1$ -out regular: True

Curvature bound: 2.000

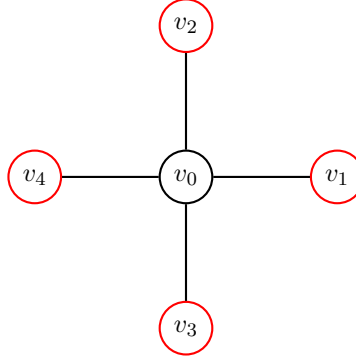

| Index | $[list_2, list_3]$                                           | Curvature | Curvature sharp |
|-------|--------------------------------------------------------------|-----------|-----------------|
| 1.1   | [[[1, 2, 3, 4], [1, 2, 3, 4], [1], [2], [3], [4]], []]       | 2.000     | True            |
| 1.2   | [[[1, 2, 3, 4], [1, 2, 3, 4], [1, 2], [3], [4]], []]         | 2.000     | True            |
| 1.3   | [[[1, 2, 3, 4], [1, 2, 3, 4], [1, 2, 3], [4]], []]           | 2.000     | True            |
| 1.4   | [[[1, 2, 3, 4], [1, 2], [1, 3], [2, 4], [3, 4]], []]         | 2.000     | True            |
| 1.5   | [[[1, 2], [1, 3], [1, 4], [2, 3], [2, 4], [3, 4]], []]       | 2.000     | True            |
| 1.6   | [[[1, 2, 3], [1, 2, 3], [1, 4], [2, 4], [3, 4]], []]         | 2.000     | True            |
| 1.7   | [[[1, 2, 3, 4], [1, 2, 3, 4], [1, 2], [3, 4]], []]           | 2.000     | True            |
| 1.8   | [[[1, 2, 3, 4], [1, 2, 3], [1, 2, 4], [3, 4]], []]           | 2.000     | True            |
| 1.9   | [[[1, 2, 3], [1, 2, 4], [1, 3, 4], [2, 3, 4]], []]           | 2.000     | True            |
| 1.10  | [[[1, 2, 3, 4], [1, 2, 3, 4], [1, 2, 3, 4]], []]             | 2.000     | True            |
| 1.11  | [[[1, 2, 3], [1, 2, 4], [1, 3], [2, 4], [3, 4]], []]         | 1.612     | False           |
| 1.12  | [[[1, 2, 3, 4], [1, 2, 3], [1, 4], [2, 4], [3]], []]         | 1.542     | False           |
| 1.13  | [[[1, 2, 3], [1, 2, 4], [1, 3, 4], [2], [3], [4]], []]       | 1.333     | False           |
| 1.14  | [[[1, 2, 3, 4], [1, 2, 3], [1, 2, 4], [3], [4]], []]         | 1.333     | False           |
| 1.15  | [[[1, 2, 3], [1, 2, 4], [1, 3, 4], [2, 3], [4]], []]         | 1.333     | False           |
| 1.16  | [[[1, 2, 3], [1, 2, 3], [1, 2, 4], [3, 4], [4]], []]         | 1.057     | False           |
| 1.17  | [[[1, 2, 3], [1, 4], [2, 4], [3, 4], [1], [2], [3]], []]     | 1.000     | False           |
| 1.18  | [[[1, 2, 3], [1, 2, 4], [1, 3], [3, 4], [2], [4]], []]       | 1.000     | False           |
| 1.19  | [[[1, 2, 3], [1, 2], [1, 4], [2, 4], [3, 4], [3]], []]       | 1.000     | False           |
| 1.20  | [[[1, 2, 3, 4], [1, 2, 3], [1, 4], [2], [3], [4]], []]       | 0.845     | False           |
| 1.21  | [[[1, 2, 3, 4], [1, 2, 3], [1, 2], [3, 4], [4]], []]         | 0.845     | False           |
| 1.22  | [[[1, 2, 3], [1, 2, 4], [3, 4], [1], [2], [3], [4]], []]     | 0.666     | False           |
| 1.23  | [[[1, 2, 3], [1, 2, 4], [1, 2], [3, 4], [3], [4]], []]       | 0.666     | False           |
| 1.24  | [[[1, 2, 3], [1, 2, 4], [3, 4], [3, 4], [1], [2]], []]       | 0.666     | False           |
| 1.25  | [[[1, 2, 3], [1, 2, 4], [1, 2], [3, 4], [3, 4]], []]         | 0.666     | False           |
| 1.26  | [[[1, 2, 3, 4], [1, 2], [1, 3], [2, 4], [3], [4]], []]       | 0.585     | False           |
| 1.27  | [[[1, 2, 3], [1, 2], [1, 3], [2, 4], [3, 4], [4]], []]       | 0.367     | False           |
| 1.28  | [[[1, 2, 3], [1, 2, 3], [1, 4], [2, 4], [3], [4]], []]       | 0.241     | False           |
| 1.29  | [[[1, 2, 3], [1, 2], [1, 4], [3, 4], [3, 4], [2]], []]       | 0.078     | False           |
| 1.30  | [[[1, 2, 3, 4], [1], [1], [2], [2], [3], [3], [4], [4]], []] | 0.000     | False           |
| 1.31  | [[[1, 2, 3, 4], [1, 2], [1], [2], [3], [3], [4], [4]], []]   | 0.000     | False           |
| 1.32  | [[[1, 2, 3, 4], [1, 2, 3], [1], [2], [3], [4], [4]], []]     | 0.000     | False           |

| Index | $[list_2, list_3]$                                                 | Curvature | Curvature sharp |
|-------|--------------------------------------------------------------------|-----------|-----------------|
| 1.33  | [[[1, 2, 3, 4], [1, 2], [1, 2], [3], [3], [4], [4]], []]           | 0.000     | False           |
| 1.34  | [[[1, 2, 3, 4], [1, 2], [1, 3], [2], [3], [4], [4]], []]           | 0.000     | False           |
| 1.35  | [[[1, 2, 3, 4], [1, 2], [3, 4], [1], [2], [3], [4]], []]           | 0.000     | False           |
| 1.36  | [[[1, 2], [1, 3], [2, 4], [3, 4], [1], [2], [3], [4]], []]         | 0.000     | False           |
| 1.37  | [[[1, 2, 3], [1, 2], [1, 4], [3, 4], [2], [3], [4]], []]           | 0.000     | False           |
| 1.38  | [[[1, 2, 3, 4], [1, 2, 3], [1, 2], [3], [4], [4]], []]             | 0.000     | False           |
| 1.39  | [[[1, 2, 3, 4], [1, 2], [1, 2], [3, 4], [3], [4]], []]             | 0.000     | False           |
| 1.40  | [[[1, 2, 3, 4], [1, 2], [1, 3], [2, 3], [4], [4]], []]             | 0.000     | False           |
| 1.41  | [[[1, 2], [1, 2], [1, 3], [2, 4], [3, 4], [3], [4]], []]           | 0.000     | False           |
| 1.42  | [[[1, 2], [1, 3], [1, 4], [2, 3], [2, 4], [3], [4]], []]           | 0.000     | False           |
| 1.43  | [[[1, 2, 3], [1, 2, 4], [1, 3], [2, 4], [3], [4]], []]             | 0.000     | False           |
| 1.44  | [[[1, 2, 3, 4], [1, 2, 3], [1, 2, 3], [4], [4]], []]               | 0.000     | False           |
| 1.45  | [[[1, 2, 3, 4], [1, 2], [1, 2], [3, 4], [3, 4]], []]               | 0.000     | False           |
| 1.46  | [[[1, 2], [1, 2], [1, 3], [2, 4], [3, 4], [3, 4]], []]             | 0.000     | False           |
| 1.47  | [[[1, 2, 3], [1, 2, 4], [1, 3], [2, 3], [4], [4]], []]             | -0.334    | False           |
| 1.48  | [[[1, 2, 3], [1, 4], [1, 4], [2, 4], [2], [3], [3]], []]           | -0.370    | False           |
| 1.49  | [[[1, 2, 3], [1, 2, 3], [1, 2, 4], [3], [4], [4]], []]             | -0.375    | False           |
| 1.50  | [[[1, 2, 3], [1, 2, 4], [1, 3], [2], [3], [4], [4]], []]           | -0.431    | False           |
| 1.51  | [[[1, 2, 3], [1, 4], [2, 4], [1], [2], [3], [3], [4]], []]         | -0.458    | False           |
| 1.52  | [[[1, 2, 3], [1, 2], [1, 4], [2, 4], [3], [3], [4]], []]           | -0.458    | False           |
| 1.53  | [[[1, 2, 3], [1, 2, 4], [1], [2], [3], [3], [4], [4]], []]         | -0.667    | False           |
| 1.54  | [[[1, 2, 3], [1, 2, 4], [1, 2], [3], [3], [4], [4]], []]           | -0.667    | False           |
| 1.55  | [[[1, 2, 3], [1, 4], [1, 4], [2], [2], [3], [3], [4]], []]         | -0.915    | False           |
| 1.56  | [[[1, 2, 3], [1, 2, 3], [1, 4], [2], [3], [4], [4]], []]           | -0.915    | False           |
| 1.57  | [[[1, 2, 3], [1, 2], [3, 4], [3, 4], [1], [2], [4]], []]           | -0.915    | False           |
| 1.58  | [[[1, 2, 3], [1, 2, 3], [1, 2], [3, 4], [4], [4]], []]             | -0.915    | False           |
| 1.59  | [[[1, 2, 3], [1, 2], [1, 2], [3, 4], [3, 4], [4]], []]             | -0.915    | False           |
| 1.60  | [[[1, 2, 3], [1, 2], [1, 3], [2, 4], [3], [4], [4]], []]           | -0.971    | False           |
| 1.61  | [[[1, 2], [1, 3], [1, 4], [2], [2], [3], [3], [4], [4]], []]       | -1.000    | False           |
| 1.62  | [[[1, 2, 3], [1, 2], [1, 4], [2], [3], [3], [4], [4]], []]         | -1.000    | False           |
| 1.63  | [[[1, 2], [1, 3], [1, 4], [2, 3], [2], [3], [4], [4]], []]         | -1.000    | False           |
| 1.64  | [[[1, 2], [1, 2], [1, 3], [2, 3], [3, 4], [4], [4]], []]           | -1.000    | False           |
| 1.65  | [[[1, 2, 3], [1, 4], [1], [2], [2], [3], [3], [4], [4]], []]       | -1.155    | False           |
| 1.66  | [[[1, 2, 3], [1, 2], [3, 4], [1], [2], [3], [4], [4]], []]         | -1.155    | False           |
| 1.67  | [[[1, 2, 3], [1, 2], [1, 2], [3, 4], [3], [4], [4]], []]           | -1.155    | False           |
| 1.68  | [[[1, 2], [1, 2], [1, 3], [2, 4], [3], [3], [4], [4]], []]         | -1.237    | False           |
| 1.69  | [[[1, 2], [1, 2], [1, 3], [3, 4], [3, 4], [2], [4]], []]           | -1.237    | False           |
| 1.70  | [[[1, 2], [1, 2], [1, 3], [3, 4], [2], [3], [4], [4]], []]         | -1.343    | False           |
| 1.71  | [[[1, 2], [1, 3], [2, 4], [1], [2], [3], [3], [4], [4]], []]       | -1.415    | False           |
| 1.72  | [[[1, 2, 3], [1], [1], [2], [2], [3], [3], [4], [4], [4]], []]     | -2.000    | False           |
| 1.73  | [[[1, 2], [1], [1], [2], [2], [3], [3], [3], [4], [4], [4]], []]   | -2.000    | False           |
| 1.74  | [[[1], [1], [1], [2], [2], [2], [3], [3], [3], [4], [4], [4]], []] | -2.000    | False           |
| 1.75  | [[[1, 2], [1, 2], [1], [2], [3], [3], [3], [4], [4], [4]], []]     | -2.000    | False           |
| 1.76  | [[[1, 2], [1, 3], [1], [2], [2], [3], [3], [4], [4], [4]], []]     | -2.000    | False           |
| 1.77  | [[[1, 2], [3, 4], [1], [1], [2], [2], [3], [3], [4], [4]], []]     | -2.000    | False           |
| 1.78  | [[[1, 2, 3], [1, 2], [1], [2], [3], [3], [4], [4], [4]], []]       | -2.000    | False           |
| 1.79  | [[[1, 2], [1, 2], [1, 2], [3], [3], [3], [4], [4], [4]], []]       | -2.000    | False           |

| Index | $[list_2, list_3]$                                           | Curvature | Curvature sharp |
|-------|--------------------------------------------------------------|-----------|-----------------|
| 1.80  | [[[1, 2], [1, 2], [1, 3], [2], [3], [3], [4], [4], [4]], []] | -2.000    | False           |
| 1.81  | [[[1, 2], [1, 2], [3, 4], [1], [2], [3], [3], [4], [4]], []] | -2.000    | False           |
| 1.82  | [[[1, 2], [1, 3], [2, 3], [1], [2], [3], [4], [4], [4]], []] | -2.000    | False           |
| 1.83  | [[[1, 2, 3], [1, 2, 3], [1], [2], [3], [4], [4], [4]], []]   | -2.000    | False           |
| 1.84  | [[[1, 2, 3], [1, 2], [1, 2], [3], [3], [4], [4], [4]], []]   | -2.000    | False           |
| 1.85  | [[[1, 2, 3], [1, 2], [1, 3], [2], [3], [4], [4], [4]], []]   | -2.000    | False           |
| 1.86  | [[[1, 2], [1, 2], [1, 2], [3, 4], [3], [3], [4], [4]], []]   | -2.000    | False           |
| 1.87  | [[[1, 2], [1, 2], [1, 3], [2, 3], [3], [4], [4], [4]], []]   | -2.000    | False           |
| 1.88  | [[[1, 2], [1, 2], [3, 4], [3, 4], [1], [2], [3], [4]], []]   | -2.000    | False           |
| 1.89  | [[[1, 2, 3], [1, 2, 3], [1, 2], [3], [4], [4], [4]], []]     | -2.000    | False           |
| 1.90  | [[[1, 2, 3], [1, 2], [1, 3], [2, 3], [4], [4], [4]], []]     | -2.000    | False           |
| 1.91  | [[[1, 2, 3], [1, 2, 3], [1, 2, 3], [4], [4], [4]], []]       | -2.000    | False           |
| 1.92  | [[[1, 2], [1, 2], [1, 2], [3, 4], [3, 4], [3], [4]], []]     | -2.000    | False           |
| 1.93  | [[[1, 2], [1, 2], [1, 2], [3, 4], [3, 4], [3, 4]], []]       | -2.000    | False           |

**2**  $list_1 = [1, 0, 0, 0, 0, 0]$

$S_1$ -out regular: False

Curvature bound: 2.250

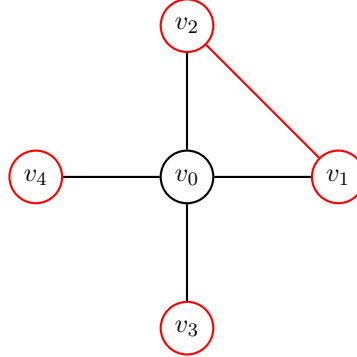

| Index | $[list_2, list_3]$                                 | Curvature | Curvature sharp |
|-------|----------------------------------------------------|-----------|-----------------|
| 2.1   | $[[[1, 3, 4], [2, 3, 4], [1, 3], [2, 4]], []]$     | 2.166     | False           |
| 2.2   | $[[[1, 2, 3, 4], [1, 3, 4], [2, 3, 4]], []]$       | 2.166     | False           |
| 2.3   | $[[[1, 3, 4], [1, 3, 4], [2, 3], [2, 4]], []]$     | 2.157     | False           |
| 2.4   | $[[[1, 2, 3, 4], [1, 2, 3, 4], [3], [4]], []]$     | 2.000     | False           |
| 2.5   | $[[[1, 2, 3, 4], [1, 3], [2, 4], [3, 4]], []]$     | 2.000     | False           |
| 2.6   | $[[[1, 3], [1, 4], [2, 3], [2, 4], [3, 4]], []]$   | 2.000     | False           |
| 2.7   | $[[[1, 2, 3, 4], [1, 2, 3, 4], [3, 4]], []]$       | 2.000     | False           |
| 2.8   | $[[[1, 3, 4], [1, 3, 4], [2, 3, 4], [2]], []]$     | 1.787     | False           |
| 2.9   | $[[[1, 2, 3], [1, 3, 4], [2, 4], [3, 4]], []]$     | 1.747     | False           |
| 2.10  | $[[[1, 2, 3, 4], [1, 3, 4], [2, 3], [4]], []]$     | 1.708     | False           |
| 2.11  | $[[[1, 2, 3], [1, 3, 4], [2, 3, 4], [4]], []]$     | 1.444     | False           |
| 2.12  | $[[[1, 3, 4], [2, 3], [2, 4], [3, 4], [1]], []]$   | 1.426     | False           |
| 2.13  | $[[[1, 3, 4], [2, 3, 4], [1, 3], [2], [4]], []]$   | 1.353     | False           |
| 2.14  | $[[[1, 2, 3, 4], [1, 3, 4], [2], [3], [4]], []]$   | 1.289     | False           |
| 2.15  | $[[[1, 2, 3, 4], [1, 3, 4], [3, 4], [2]], []]$     | 1.289     | False           |
| 2.16  | $[[[1, 3, 4], [1, 3], [2, 4], [3, 4], [2]], []]$   | 1.164     | False           |
| 2.17  | $[[[1, 2, 3], [1, 4], [2, 4], [3, 4], [3]], []]$   | 1.120     | False           |
| 2.18  | $[[[1, 3, 4], [1, 3], [2, 3], [2, 4], [4]], []]$   | 1.106     | False           |
| 2.19  | $[[[1, 2, 3], [1, 3, 4], [2, 4], [3], [4]], []]$   | 1.056     | False           |
| 2.20  | $[[[1, 3, 4], [2, 3], [2, 4], [1], [3], [4]], []]$ | 1.000     | False           |
| 2.21  | $[[[1, 2, 3, 4], [1, 2, 3], [3, 4], [4]], []]$     | 1.000     | False           |
| 2.22  | $[[[1, 3, 4], [1, 3, 4], [2, 3], [2], [4]], []]$   | 0.938     | False           |
| 2.23  | $[[[1, 3], [1, 3], [2, 4], [2, 4], [3, 4]], []]$   | 0.891     | False           |
| 2.24  | $[[[1, 3, 4], [2, 3, 4], [1], [2], [3], [4]], []]$ | 0.871     | False           |
| 2.25  | $[[[1, 2, 3], [1, 2, 4], [3, 4], [3], [4]], []]$   | 0.871     | False           |
| 2.26  | $[[[1, 3, 4], [2, 3, 4], [1, 2], [3], [4]], []]$   | 0.871     | False           |
| 2.27  | $[[[1, 3, 4], [2, 3, 4], [3, 4], [1], [2]], []]$   | 0.871     | False           |
| 2.28  | $[[[1, 2, 3], [1, 2, 4], [3, 4], [3, 4]], []]$     | 0.871     | False           |
| 2.29  | $[[[1, 3, 4], [2, 3, 4], [1, 2], [3, 4]], []]$     | 0.871     | False           |
| 2.30  | $[[[1, 2, 3, 4], [1, 3], [3, 4], [2], [4]], []]$   | 0.842     | False           |
| 2.31  | $[[[1, 2, 3, 4], [1, 3], [2, 4], [3], [4]], []]$   | 0.787     | False           |
| 2.32  | $[[[1, 3, 4], [1, 3], [2, 4], [2, 4], [3]], []]$   | 0.615     | False           |

| Index | $[list_2, list_3]$                                   | Curvature | Curvature sharp |
|-------|------------------------------------------------------|-----------|-----------------|
| 2.33  | [[[1, 3, 4], [1, 3], [2, 4], [2], [3], [4]], []]     | 0.614     | False           |
| 2.34  | [[[1, 2, 3], [1, 3], [2, 4], [3, 4], [4]], []]       | 0.561     | False           |
| 2.35  | [[[1, 3], [1, 3], [2, 4], [3, 4], [2], [4]], []]     | 0.543     | False           |
| 2.36  | [[[1, 3], [1, 4], [2, 3], [3, 4], [2], [4]], []]     | 0.427     | False           |
| 2.37  | [[[1, 2, 3], [1, 4], [3, 4], [3, 4], [2]], []]       | 0.404     | False           |
| 2.38  | [[[1, 2, 3], [1, 4], [3, 4], [2], [3], [4]], []]     | 0.321     | False           |
| 2.39  | [[[1, 2, 3], [1, 3, 4], [3, 4], [2], [4]], []]       | 0.321     | False           |
| 2.40  | [[[1, 3, 4], [1, 2], [2, 3], [3, 4], [4]], []]       | 0.294     | False           |
| 2.41  | [[[1, 3, 4], [2, 3], [3, 4], [1], [2], [4]], []]     | 0.278     | False           |
| 2.42  | [[[1, 2, 3, 4], [3, 4], [1], [2], [3], [4]], []]     | 0.219     | False           |
| 2.43  | [[[1, 3], [2, 4], [3, 4], [1], [2], [3], [4]], []]   | 0.219     | False           |
| 2.44  | [[[1, 2, 3, 4], [1, 2], [3, 4], [3], [4]], []]       | 0.219     | False           |
| 2.45  | [[[1, 2, 3, 4], [3, 4], [3, 4], [1], [2]], []]       | 0.219     | False           |
| 2.46  | [[[1, 2], [1, 3], [2, 4], [3, 4], [3], [4]], []]     | 0.219     | False           |
| 2.47  | [[[1, 3], [2, 4], [3, 4], [3, 4], [1], [2]], []]     | 0.219     | False           |
| 2.48  | [[[1, 2, 3, 4], [1, 2], [3, 4], [3, 4]], []]         | 0.219     | False           |
| 2.49  | [[[1, 2], [1, 3], [2, 4], [3, 4], [3, 4]], []]       | 0.219     | False           |
| 2.50  | [[[1, 2, 3, 4], [1, 3], [2, 3], [4], [4]], []]       | 0.070     | False           |
| 2.51  | [[[1, 2, 3, 4], [1, 2, 3], [3], [4], [4]], []]       | 0.068     | False           |
| 2.52  | [[[1, 2, 3, 4], [1, 3], [2], [3], [4], [4]], []]     | 0.066     | False           |
| 2.53  | [[[1, 2, 3, 4], [1], [2], [3], [3], [4], [4]], []]   | 0.000     | False           |
| 2.54  | [[[1, 2, 3, 4], [1, 2], [3], [3], [4], [4]], []]     | 0.000     | False           |
| 2.55  | [[[1, 3], [1, 4], [2, 3], [2, 4], [3], [4]], []]     | 0.000     | False           |
| 2.56  | [[[1, 3, 4], [1, 3, 4], [2], [2], [3], [4]], []]     | -0.031    | False           |
| 2.57  | [[[1, 3, 4], [1, 3, 4], [3, 4], [2], [2]], []]       | -0.031    | False           |
| 2.58  | [[[1, 2, 3], [1, 3, 4], [2, 3], [4], [4]], []]       | -0.210    | False           |
| 2.59  | [[[1, 3, 4], [2, 3], [2, 3], [1], [4], [4]], []]     | -0.218    | False           |
| 2.60  | [[[1, 3, 4], [1, 2], [2, 3], [3], [4], [4]], []]     | -0.226    | False           |
| 2.61  | [[[1, 3, 4], [1, 3], [3, 4], [2], [2], [4]], []]     | -0.233    | False           |
| 2.62  | [[[1, 2, 3], [1, 3, 4], [2], [3], [4], [4]], []]     | -0.247    | False           |
| 2.63  | [[[1, 3, 4], [1, 3], [2, 3], [2], [4], [4]], []]     | -0.247    | False           |
| 2.64  | [[[1, 3, 4], [2, 3], [1], [2], [3], [4], [4]], []]   | -0.250    | False           |
| 2.65  | [[[1, 3], [1, 4], [3, 4], [2], [2], [3], [4]], []]   | -0.301    | False           |
| 2.66  | [[[1, 3], [1, 4], [3, 4], [3, 4], [2], [2]], []]     | -0.301    | False           |
| 2.67  | [[[1, 3, 4], [1, 3], [2], [2], [3], [4], [4]], []]   | -0.409    | False           |
| 2.68  | [[[1, 2, 3], [1, 4], [2, 4], [3], [3], [4]], []]     | -0.445    | False           |
| 2.69  | [[[1, 3, 4], [1, 2], [2], [3], [3], [4], [4]], []]   | -0.593    | False           |
| 2.70  | [[[1, 3, 4], [1, 2], [3, 4], [2], [3], [4]], []]     | -0.593    | False           |
| 2.71  | [[[1, 3, 4], [1, 2], [3, 4], [3, 4], [2]], []]       | -0.593    | False           |
| 2.72  | [[[1, 2, 3], [1, 2, 4], [3], [3], [4], [4]], []]     | -0.667    | False           |
| 2.73  | [[[1, 3, 4], [1], [2], [2], [3], [3], [4], [4]], []] | -0.670    | False           |
| 2.74  | [[[1, 3, 4], [3, 4], [1], [2], [2], [3], [4]], []]   | -0.670    | False           |
| 2.75  | [[[1, 3, 4], [3, 4], [3, 4], [1], [2], [2]], []]     | -0.670    | False           |
| 2.76  | [[[1, 2, 3], [3, 4], [3, 4], [1], [2], [4]], []]     | -0.702    | False           |
| 2.77  | [[[1, 2, 3], [1, 2], [3, 4], [3, 4], [4]], []]       | -0.702    | False           |
| 2.78  | [[[1, 3], [1, 3], [2, 4], [2, 4], [3], [4]], []]     | -0.761    | False           |
| 2.79  | [[[1, 2, 3], [1, 2, 3], [3, 4], [4], [4]], []]       | -0.784    | False           |

| Index | $[list_2, list_3]$                                       | Curvature | Curvature sharp |
|-------|----------------------------------------------------------|-----------|-----------------|
| 2.80  | [[[1, 2, 3], [1, 3], [3, 4], [2], [4], [4]], []]         | -0.822    | False           |
| 2.81  | [[[1, 3], [1, 3], [2, 3], [2, 4], [4], [4]], []]         | -0.840    | False           |
| 2.82  | [[[1, 3], [2, 3], [3, 4], [1], [2], [4], [4]], []]       | -0.851    | False           |
| 2.83  | [[[1, 2], [1, 3], [2, 3], [3, 4], [4], [4]], []]         | -0.851    | False           |
| 2.84  | [[[1, 3], [1, 4], [2, 3], [2], [3], [4], [4]], []]       | -0.858    | False           |
| 2.85  | [[[1, 2, 3], [1, 3], [2, 4], [3], [4], [4]], []]         | -0.858    | False           |
| 2.86  | [[[1, 3], [1, 3], [3, 4], [2], [2], [4], [4]], []]       | -0.927    | False           |
| 2.87  | [[[1, 2, 3], [1, 4], [2], [3], [3], [4], [4]], []]       | -0.937    | False           |
| 2.88  | [[[1, 2], [1, 3], [3, 4], [3, 4], [2], [4]], []]         | -0.976    | False           |
| 2.89  | [[[1, 2, 3], [3, 4], [1], [2], [3], [4], [4]], []]       | -0.977    | False           |
| 2.90  | [[[1, 2, 3], [1, 2], [3, 4], [3], [4], [4]], []]         | -0.977    | False           |
| 2.91  | [[[1, 3], [1, 4], [2], [2], [3], [3], [4], [4]], []]     | -1.000    | False           |
| 2.92  | [[[1, 3], [3, 4], [3, 4], [1], [2], [2], [4]], []]       | -1.006    | False           |
| 2.93  | [[[1, 3], [1, 3], [2, 4], [2], [3], [4], [4]], []]       | -1.058    | False           |
| 2.94  | [[[1, 2], [1, 3], [3, 4], [2], [3], [4], [4]], []]       | -1.118    | False           |
| 2.95  | [[[1, 3], [3, 4], [1], [2], [2], [3], [4], [4]], []]     | -1.135    | False           |
| 2.96  | [[[1, 2], [1, 3], [2, 4], [3], [3], [4], [4]], []]       | -1.151    | False           |
| 2.97  | [[[1, 3], [2, 4], [1], [2], [3], [3], [4], [4]], []]     | -1.213    | False           |
| 2.98  | [[[3, 4], [1], [1], [2], [2], [3], [3], [4], [4]], []]   | -1.766    | False           |
| 2.99  | [[[1, 2], [3, 4], [1], [2], [3], [3], [4], [4]], []]     | -1.766    | False           |
| 2.100 | [[[3, 4], [3, 4], [1], [1], [2], [2], [3], [4]], []]     | -1.766    | False           |
| 2.101 | [[[1, 2], [1, 2], [3, 4], [3], [3], [4], [4]], []]       | -1.766    | False           |
| 2.102 | [[[1, 2], [3, 4], [3, 4], [1], [2], [3], [4]], []]       | -1.766    | False           |
| 2.103 | [[[3, 4], [3, 4], [3, 4], [1], [1], [2], [2]], []]       | -1.766    | False           |
| 2.104 | [[[1, 2], [1, 2], [3, 4], [3, 4], [3], [4]], []]         | -1.766    | False           |
| 2.105 | [[[1, 2], [3, 4], [3, 4], [3, 4], [1], [2]], []]         | -1.766    | False           |
| 2.106 | [[[1, 2], [1, 2], [3, 4], [3, 4], [3, 4]], []]           | -1.766    | False           |
| 2.107 | [[[1, 3], [1, 3], [2, 3], [2], [4], [4], [4]], []]       | -1.925    | False           |
| 2.108 | [[[1, 2, 3], [1, 2, 3], [3], [4], [4], [4]], []]         | -1.925    | False           |
| 2.109 | [[[1, 2, 3], [1, 3], [2, 3], [4], [4], [4]], []]         | -1.925    | False           |
| 2.110 | [[[1, 3], [2, 3], [1], [2], [3], [4], [4], [4]], []]     | -1.926    | False           |
| 2.111 | [[[1, 2, 3], [1, 3], [2], [3], [4], [4], [4]], []]       | -1.926    | False           |
| 2.112 | [[[1, 2], [1, 3], [2, 3], [3], [4], [4], [4]], []]       | -1.926    | False           |
| 2.113 | [[[1, 3], [1, 3], [2], [2], [3], [4], [4], [4]], []]     | -1.927    | False           |
| 2.114 | [[[1, 2, 3], [1], [2], [3], [3], [4], [4], [4]], []]     | -1.928    | False           |
| 2.115 | [[[1, 2, 3], [1, 2], [3], [3], [4], [4], [4]], []]       | -1.928    | False           |
| 2.116 | [[[1, 2], [1, 3], [2], [3], [3], [4], [4], [4]], []]     | -1.930    | False           |
| 2.117 | [[[1, 3], [1], [2], [2], [3], [3], [4], [4], [4]], []]   | -1.931    | False           |
| 2.118 | [[[1, 2], [1], [2], [3], [3], [3], [4], [4], [4]], []]   | -2.000    | False           |
| 2.119 | [[[1], [1], [2], [2], [3], [3], [3], [4], [4], [4]], []] | -2.000    | False           |
| 2.120 | [[[1, 2], [1, 2], [3], [3], [3], [4], [4], [4]], []]     | -2.000    | False           |

**3**  $list_1 = [1, 0, 0, 0, 0, 1]$

$S_1$ -out regular: True

Curvature bound: 2.500

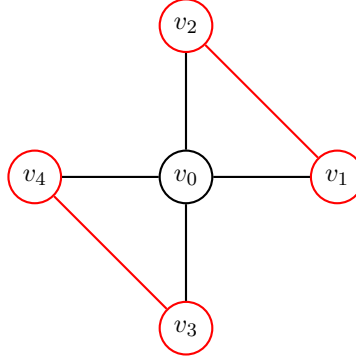

| Index | $[list_2, list_3]$                           | Curvature | Curvature sharp |
|-------|----------------------------------------------|-----------|-----------------|
| 3.1   | $[[[1, 2, 3, 4], [1, 3], [2, 4]], []]$       | 2.500     | True            |
| 3.2   | $[[[1, 3], [1, 3], [2, 4], [2, 4]], []]$     | 2.500     | True            |
| 3.3   | $[[[1, 3], [1, 4], [2, 3], [2, 4]], []]$     | 2.500     | True            |
| 3.4   | $[[[1, 2, 3, 4], [1, 2, 3, 4]], []]$         | 2.500     | True            |
| 3.5   | $[[[1, 2, 3], [1, 3, 4], [2, 4]], []]$       | 2.139     | False           |
| 3.6   | $[[[1, 2, 3], [1, 4], [2, 4], [3]], []]$     | 1.741     | False           |
| 3.7   | $[[[1, 2, 3, 4], [1, 2, 3], [4]], []]$       | 1.585     | False           |
| 3.8   | $[[[1, 2, 3], [1, 3], [2, 4], [4]], []]$     | 1.470     | False           |
| 3.9   | $[[[1, 2, 3, 4], [1, 3], [2], [4]], []]$     | 1.263     | False           |
| 3.10  | $[[[1, 3], [1, 3], [2, 4], [2], [4]], []]$   | 1.263     | False           |
| 3.11  | $[[[1, 2, 3], [1, 2, 4], [3], [4]], []]$     | 1.166     | False           |
| 3.12  | $[[[1, 2, 3], [1, 2, 4], [3, 4]], []]$       | 1.166     | False           |
| 3.13  | $[[[1, 3], [1, 4], [2, 3], [2], [4]], []]$   | 1.085     | False           |
| 3.14  | $[[[1, 2, 3], [1, 3, 4], [2], [4]], []]$     | 0.762     | False           |
| 3.15  | $[[[1, 2, 3], [1, 4], [3, 4], [2]], []]$     | 0.696     | False           |
| 3.16  | $[[[1, 2, 3], [1, 4], [2], [3], [4]], []]$   | 0.683     | False           |
| 3.17  | $[[[1, 2, 3, 4], [1], [2], [3], [4]], []]$   | 0.500     | False           |
| 3.18  | $[[[1, 3], [2, 4], [1], [2], [3], [4]], []]$ | 0.500     | False           |
| 3.19  | $[[[1, 2, 3, 4], [1, 2], [3], [4]], []]$     | 0.500     | False           |
| 3.20  | $[[[1, 2], [1, 3], [2, 4], [3], [4]], []]$   | 0.500     | False           |
| 3.21  | $[[[1, 2, 3, 4], [1, 2], [3, 4]], []]$       | 0.500     | False           |
| 3.22  | $[[[1, 2], [1, 3], [2, 4], [3, 4]], []]$     | 0.500     | False           |
| 3.23  | $[[[1, 2, 3], [1, 2, 3], [4], [4]], []]$     | 0.190     | False           |
| 3.24  | $[[[1, 2, 3], [1, 3], [2], [4], [4]], []]$   | 0.036     | False           |
| 3.25  | $[[[1, 3], [1, 4], [2], [2], [3], [4]], []]$ | -0.062    | False           |
| 3.26  | $[[[1, 2], [1, 3], [2, 3], [4], [4]], []]$   | -0.062    | False           |
| 3.27  | $[[[1, 3], [1, 3], [2], [2], [4], [4]], []]$ | -0.329    | False           |
| 3.28  | $[[[1, 2, 3], [3, 4], [1], [2], [4]], []]$   | -0.329    | False           |
| 3.29  | $[[[1, 2, 3], [1, 2], [3, 4], [4]], []]$     | -0.329    | False           |
| 3.30  | $[[[1, 2, 3], [1], [2], [3], [4], [4]], []]$ | -0.415    | False           |
| 3.31  | $[[[1, 2, 3], [1, 2], [3], [4], [4]], []]$   | -0.415    | False           |
| 3.32  | $[[[1, 2], [1, 3], [3, 4], [2], [4]], []]$   | -0.663    | False           |



| Index | $[list_2, list_3]$                             | Curvature | Curvature sharp |
|-------|------------------------------------------------|-----------|-----------------|
| 3.33  | [[[1, 2], [1, 3], [2], [3], [4], [4]], []]     | -0.702    | False           |
| 3.34  | [[[1, 3], [1], [2], [2], [3], [4], [4]], []]   | -0.737    | False           |
| 3.35  | [[[1, 2], [1], [2], [3], [3], [4], [4]], []]   | -1.500    | False           |
| 3.36  | [[[1], [1], [2], [2], [3], [3], [4], [4]], []] | -1.500    | False           |
| 3.37  | [[[1, 2], [1, 2], [3], [3], [4], [4]], []]     | -1.500    | False           |
| 3.38  | [[[1, 2], [3, 4], [1], [2], [3], [4]], []]     | -1.500    | False           |
| 3.39  | [[[1, 2], [1, 2], [3, 4], [3], [4]], []]       | -1.500    | False           |
| 3.40  | [[[1, 2], [1, 2], [3, 4], [3, 4]], []]         | -1.500    | False           |

4  $list_1 = [1, 1, 0, 0, 0, 0]$

$S_1$ -out regular: False

Curvature bound: 2.500

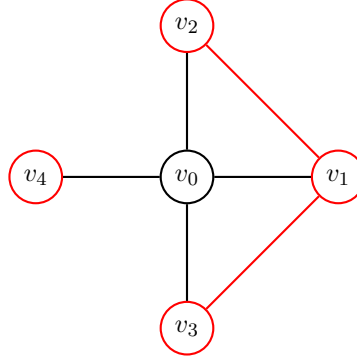

| Index | $[list_2, list_3]$                           | Curvature | Curvature sharp |
|-------|----------------------------------------------|-----------|-----------------|
| 4.1   | $[[[2, 3, 4], [2, 3, 4], [1, 4]], []]$       | 2.357     | False           |
| 4.2   | $[[[1, 2, 4], [2, 3, 4], [3, 4]], []]$       | 2.302     | False           |
| 4.3   | $[[[1, 2, 3, 4], [2, 4], [3, 4]], []]$       | 2.254     | False           |
| 4.4   | $[[[1, 4], [2, 3], [2, 4], [3, 4]], []]$     | 2.000     | False           |
| 4.5   | $[[[2, 3, 4], [1, 4], [2, 4], [3]], []]$     | 1.879     | False           |
| 4.6   | $[[[2, 3, 4], [2, 4], [3, 4], [1]], []]$     | 1.814     | False           |
| 4.7   | $[[[1, 2, 3, 4], [2, 3, 4], [4]], []]$       | 1.764     | False           |
| 4.8   | $[[[1, 2, 4], [2, 4], [3, 4], [3]], []]$     | 1.746     | False           |
| 4.9   | $[[[1, 4], [2, 4], [3, 4], [2], [3]], []]$   | 1.500     | False           |
| 4.10  | $[[[1, 2, 4], [2, 3, 4], [3], [4]], []]$     | 1.467     | False           |
| 4.11  | $[[[2, 3, 4], [2, 3, 4], [1], [4]], []]$     | 1.295     | False           |
| 4.12  | $[[[1, 2, 4], [3, 4], [3, 4], [2]], []]$     | 1.204     | False           |
| 4.13  | $[[[2, 3, 4], [1, 4], [2], [3], [4]], []]$   | 1.181     | False           |
| 4.14  | $[[[1, 2, 4], [2, 3], [3, 4], [4]], []]$     | 1.181     | False           |
| 4.15  | $[[[2, 3, 4], [1, 4], [2, 3], [4]], []]$     | 1.181     | False           |
| 4.16  | $[[[1, 2], [2, 4], [3, 4], [3, 4]], []]$     | 1.110     | False           |
| 4.17  | $[[[2, 4], [2, 4], [3, 4], [1], [3]], []]$   | 1.091     | False           |
| 4.18  | $[[[1, 2, 3, 4], [2, 4], [3], [4]], []]$     | 1.081     | False           |
| 4.19  | $[[[1, 2, 4], [3, 4], [2], [3], [4]], []]$   | 1.075     | False           |
| 4.20  | $[[[2, 3, 4], [2, 4], [1], [3], [4]], []]$   | 0.746     | False           |
| 4.21  | $[[[2, 3, 4], [1, 2], [3, 4], [4]], []]$     | 0.746     | False           |
| 4.22  | $[[[1, 2, 3], [2, 4], [3, 4], [4]], []]$     | 0.674     | False           |
| 4.23  | $[[[1, 2], [2, 4], [3, 4], [3], [4]], []]$   | 0.653     | False           |
| 4.24  | $[[[2, 4], [3, 4], [1], [2], [3], [4]], []]$ | 0.626     | False           |
| 4.25  | $[[[2, 3], [2, 4], [3, 4], [1], [4]], []]$   | 0.626     | False           |
| 4.26  | $[[[1, 4], [2, 3], [2, 4], [3], [4]], []]$   | 0.448     | False           |
| 4.27  | $[[[1, 2, 3, 4], [2], [3], [4], [4]], []]$   | 0.130     | False           |
| 4.28  | $[[[1, 2, 3, 4], [2, 3], [4], [4]], []]$     | 0.130     | False           |
| 4.29  | $[[[1, 4], [2, 4], [2, 4], [3], [3]], []]$   | 0.107     | False           |
| 4.30  | $[[[1, 2, 4], [2, 4], [3], [3], [4]], []]$   | 0.012     | False           |
| 4.31  | $[[[1, 4], [2, 4], [2], [3], [3], [4]], []]$ | 0.010     | False           |
| 4.32  | $[[[1, 2, 3], [2, 3, 4], [4], [4]], []]$     | -0.127    | False           |

| Index | $[list_2, list_3]$                               | Curvature | Curvature sharp |
|-------|--------------------------------------------------|-----------|-----------------|
| 4.33  | $[[[2, 3, 4], [1, 2], [3], [4], [4]], []]$       | -0.132    | False           |
| 4.34  | $[[[2, 3, 4], [1], [2], [3], [4], [4]], []]$     | -0.142    | False           |
| 4.35  | $[[[2, 3, 4], [2, 3], [1], [4], [4]], []]$       | -0.142    | False           |
| 4.36  | $[[[1, 2, 4], [2, 3], [3], [4], [4]], []]$       | -0.219    | False           |
| 4.37  | $[[[1, 2, 4], [2], [3], [3], [4], [4]], []]$     | -0.355    | False           |
| 4.38  | $[[[1, 2], [3, 4], [3, 4], [2], [4]], []]$       | -0.441    | False           |
| 4.39  | $[[[2, 4], [2, 4], [1], [3], [3], [4]], []]$     | -0.533    | False           |
| 4.40  | $[[[1, 4], [2], [2], [3], [3], [4], [4]], []]$   | -0.702    | False           |
| 4.41  | $[[[1, 4], [2, 3], [2], [3], [4], [4]], []]$     | -0.702    | False           |
| 4.42  | $[[[1, 4], [2, 3], [2, 3], [4], [4]], []]$       | -0.702    | False           |
| 4.43  | $[[[1, 2], [2, 3], [3, 4], [4], [4]], []]$       | -0.717    | False           |
| 4.44  | $[[[1, 2, 3], [2, 4], [3], [4], [4]], []]$       | -0.718    | False           |
| 4.45  | $[[[2, 3], [2, 4], [1], [3], [4], [4]], []]$     | -0.722    | False           |
| 4.46  | $[[[1, 2], [2, 4], [3], [3], [4], [4]], []]$     | -0.814    | False           |
| 4.47  | $[[[1, 2], [3, 4], [2], [3], [4], [4]], []]$     | -0.854    | False           |
| 4.48  | $[[[2, 4], [1], [2], [3], [3], [4], [4]], []]$   | -0.889    | False           |
| 4.49  | $[[[1, 2, 3], [2], [3], [4], [4], [4]], []]$     | -1.854    | False           |
| 4.50  | $[[[1, 2], [2], [3], [3], [4], [4], [4]], []]$   | -1.854    | False           |
| 4.51  | $[[[1, 2], [2, 3], [3], [4], [4], [4]], []]$     | -1.854    | False           |
| 4.52  | $[[[1, 2, 3], [2, 3], [4], [4], [4]], []]$       | -1.854    | False           |
| 4.53  | $[[[2, 3], [1], [2], [3], [4], [4], [4]], []]$   | -1.855    | False           |
| 4.54  | $[[[1], [2], [2], [3], [3], [4], [4], [4]], []]$ | -1.855    | False           |
| 4.55  | $[[[2, 3], [2, 3], [1], [4], [4], [4]], []]$     | -1.855    | False           |

**5**  $list_1 = [1, 1, 1, 0, 0, 0]$

$S_1$ -out regular: False

Curvature bound: 2.750

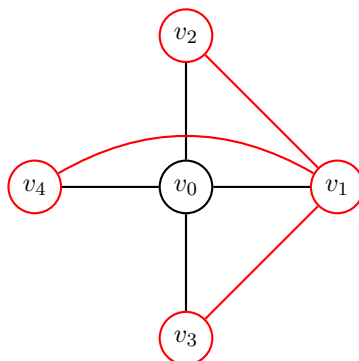

| Index | $[list_2, list_3]$                     | Curvature | Curvature sharp |
|-------|----------------------------------------|-----------|-----------------|
| 5.1   | $[[[2, 3], [2, 4], [3, 4]], []]$       | 2.708     | False           |
| 5.2   | $[[[2, 3, 4], [2, 3, 4]], []]$         | 2.708     | False           |
| 5.3   | $[[[2, 3, 4], [2], [3], [4]], []]$     | 2.500     | False           |
| 5.4   | $[[[2, 3, 4], [2, 3], [4]], []]$       | 2.500     | False           |
| 5.5   | $[[[2, 3], [2, 4], [3], [4]], []]$     | 1.500     | False           |
| 5.6   | $[[[2, 3], [2], [3], [4], [4]], []]$   | 0.500     | False           |
| 5.7   | $[[[2], [2], [3], [3], [4], [4]], []]$ | 0.500     | False           |
| 5.8   | $[[[2, 3], [2, 3], [4], [4]], []]$     | 0.500     | False           |

**6**  $list_1 = [1, 1, 0, 1, 0, 0]$

$S_1$ -out regular: False

Curvature bound: 2.750

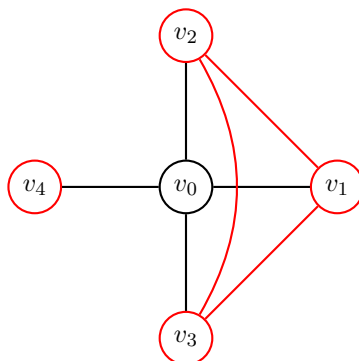

| Index | $[list_2, list_3]$                     | Curvature | Curvature sharp |
|-------|----------------------------------------|-----------|-----------------|
| 6.1   | $[[[1, 4], [2, 4], [3, 4]], []]$       | 2.000     | False           |
| 6.2   | $[[[1, 2, 4], [3, 4], [4]], []]$       | 1.217     | False           |
| 6.3   | $[[[1, 4], [2, 4], [3], [4]], []]$     | 0.638     | False           |
| 6.4   | $[[[1, 2, 3, 4], [4], [4]], []]$       | 0.177     | False           |
| 6.5   | $[[[1, 2, 4], [3], [4], [4]], []]$     | -0.112    | False           |
| 6.6   | $[[[1, 4], [2], [3], [4], [4]], []]$   | -0.614    | False           |
| 6.7   | $[[[1, 2], [3, 4], [4], [4]], []]$     | -0.614    | False           |
| 6.8   | $[[[1, 2, 3], [4], [4], [4]], []]$     | -1.792    | False           |
| 6.9   | $[[[1, 2], [3], [4], [4], [4]], []]$   | -1.792    | False           |
| 6.10  | $[[[1], [2], [3], [4], [4], [4]], []]$ | -1.792    | False           |

**7**  $list_1 = [1, 1, 0, 0, 1, 0]$

$S_1$ -out regular: False

Curvature bound: 2.750

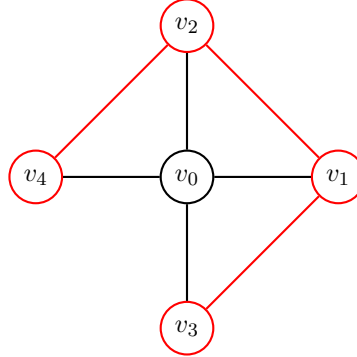

| Index | $[list_2, list_3]$                     | Curvature | Curvature sharp |
|-------|----------------------------------------|-----------|-----------------|
| 7.1   | $[[[1, 3, 4], [2, 3, 4]], []]$         | 2.726     | False           |
| 7.2   | $[[[1, 2, 3, 4], [3, 4]], []]$         | 2.719     | False           |
| 7.3   | $[[[1, 4], [2, 3], [3, 4]], []]$       | 2.719     | False           |
| 7.4   | $[[[1, 3, 4], [3, 4], [2]], []]$       | 2.622     | False           |
| 7.5   | $[[[3, 4], [3, 4], [1], [2]], []]$     | 2.500     | False           |
| 7.6   | $[[[1, 2], [3, 4], [3, 4]], []]$       | 2.500     | False           |
| 7.7   | $[[[1, 3, 4], [2, 3], [4]], []]$       | 2.278     | False           |
| 7.8   | $[[[1, 2, 3], [3, 4], [4]], []]$       | 1.944     | False           |
| 7.9   | $[[[1, 4], [3, 4], [2], [3]], []]$     | 1.816     | False           |
| 7.10  | $[[[1, 2, 3, 4], [3], [4]], []]$       | 1.739     | False           |
| 7.11  | $[[[1, 2], [3, 4], [3], [4]], []]$     | 1.739     | False           |
| 7.12  | $[[[1, 3], [2, 4], [3, 4]], []]$       | 1.500     | False           |
| 7.13  | $[[[1, 3, 4], [2, 4], [3]], []]$       | 1.473     | False           |
| 7.14  | $[[[1, 3, 4], [2], [3], [4]], []]$     | 1.463     | False           |
| 7.15  | $[[[1, 3], [3, 4], [2], [4]], []]$     | 1.429     | False           |
| 7.16  | $[[[3, 4], [1], [2], [3], [4]], []]$   | 1.391     | False           |
| 7.17  | $[[[1, 4], [2, 3], [3], [4]], []]$     | 1.287     | False           |
| 7.18  | $[[[1, 3], [2, 3], [4], [4]], []]$     | 0.337     | False           |
| 7.19  | $[[[1, 2, 3], [3], [4], [4]], []]$     | 0.328     | False           |
| 7.20  | $[[[1, 4], [2], [3], [3], [4]], []]$   | 0.315     | False           |
| 7.21  | $[[[1, 3], [2, 4], [3], [4]], []]$     | 0.000     | False           |
| 7.22  | $[[[1, 2], [3], [3], [4], [4]], []]$   | -0.067    | False           |
| 7.23  | $[[[1, 3], [2], [3], [4], [4]], []]$   | -0.148    | False           |
| 7.24  | $[[[1], [2], [3], [3], [4], [4]], []]$ | -0.261    | False           |

8  $list_1 = [1, 1, 0, 0, 1, 1]$

$S_1$ -out regular: True

Curvature bound: 3.000

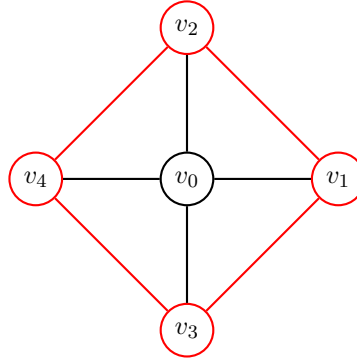

| Index | $[list_2, list_3]$           | Curvature | Curvature sharp |
|-------|------------------------------|-----------|-----------------|
| 8.1   | $[[[1, 2, 3, 4]], []]$       | 3.000     | True            |
| 8.2   | $[[[1, 2, 3], [4]], []]$     | 3.000     | True            |
| 8.3   | $[[[1, 2], [3], [4]], []]$   | 3.000     | True            |
| 8.4   | $[[[1, 4], [2], [3]], []]$   | 3.000     | True            |
| 8.5   | $[[[1], [2], [3], [4]], []]$ | 3.000     | True            |
| 8.6   | $[[[1, 2], [3, 4]], []]$     | 3.000     | True            |
| 8.7   | $[[[1, 4], [2, 3]], []]$     | 3.000     | True            |

**9**  $list_1 = [1, 1, 1, 1, 0, 0]$

$S_1$ -out regular: False

Curvature bound: 3.000

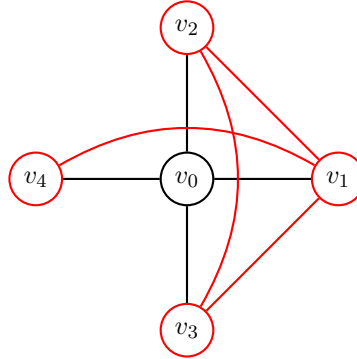

| Index | $[list_2, list_3]$           | Curvature | Curvature sharp |
|-------|------------------------------|-----------|-----------------|
| 9.1   | $[[[2, 4], [3, 4]], []]$     | 2.920     | False           |
| 9.2   | $[[[2, 3, 4], [4]], []]$     | 2.558     | False           |
| 9.3   | $[[[2, 4], [3], [4]], []]$   | 1.913     | False           |
| 9.4   | $[[[2, 3], [4], [4]], []]$   | 0.645     | False           |
| 9.5   | $[[[2], [3], [4], [4]], []]$ | 0.645     | False           |



**10**  $list_1 = [1, 1, 1, 1, 1, 0]$

$S_1$ -out regular: False

Curvature bound: 3.250

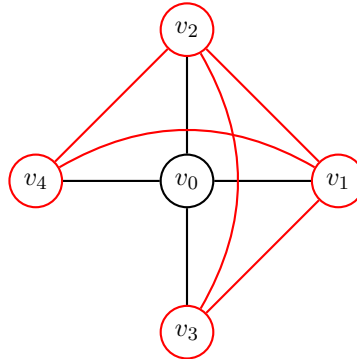

| Index | $[list_2, list_3]$ | Curvature | Curvature sharp |
|-------|--------------------|-----------|-----------------|
| 10.1  | $[[[3, 4]], []]$   | 3.234     | False           |
| 10.2  | $[[[3], [4]], []]$ | 3.000     | False           |

**11**     $list_1 = [1, 1, 1, 1, 1, 1]$

$S_1$ -out regular: True

Curvature bound: 3.500

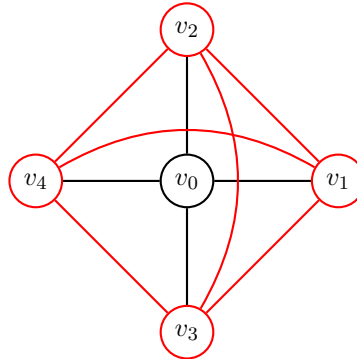

| Index | $[list_2, list_3]$   | Curvature | Curvature sharp |
|-------|----------------------|-----------|-----------------|
| 11.1  | $[\square, \square]$ | 3.500     | True            |

## Curvature Sharp Graphs

Total: 22

| Index | Incomplete 2-ball                                                          | Curvature |
|-------|----------------------------------------------------------------------------|-----------|
| 1.1   | [[0, 0, 0, 0, 0, 0], [[1, 2, 3, 4], [1, 2, 3, 4], [1], [2], [3], [4]], []] | 2.000     |
| 1.2   | [[0, 0, 0, 0, 0, 0], [[1, 2, 3, 4], [1, 2, 3, 4], [1, 2], [3], [4]], []]   | 2.000     |
| 1.3   | [[0, 0, 0, 0, 0, 0], [[1, 2, 3, 4], [1, 2, 3, 4], [1, 2, 3], [4]], []]     | 2.000     |
| 1.4   | [[0, 0, 0, 0, 0, 0], [[1, 2, 3, 4], [1, 2], [1, 3], [2, 4], [3, 4]], []]   | 2.000     |
| 1.5   | [[0, 0, 0, 0, 0, 0], [[1, 2], [1, 3], [1, 4], [2, 3], [2, 4], [3, 4]], []] | 2.000     |
| 1.6   | [[0, 0, 0, 0, 0, 0], [[1, 2, 3], [1, 2, 3], [1, 4], [2, 4], [3, 4]], []]   | 2.000     |
| 1.7   | [[0, 0, 0, 0, 0, 0], [[1, 2, 3, 4], [1, 2, 3, 4], [1, 2], [3, 4]], []]     | 2.000     |
| 1.8   | [[0, 0, 0, 0, 0, 0], [[1, 2, 3, 4], [1, 2, 3], [1, 2, 4], [3, 4]], []]     | 2.000     |
| 1.9   | [[0, 0, 0, 0, 0, 0], [[1, 2, 3], [1, 2, 4], [1, 3, 4], [2, 3, 4]], []]     | 2.000     |
| 1.10  | [[0, 0, 0, 0, 0, 0], [[1, 2, 3, 4], [1, 2, 3, 4], [1, 2, 3, 4]], []]       | 2.000     |
| 3.1   | [[1, 0, 0, 0, 0, 1], [[1, 2, 3, 4], [1, 3], [2, 4]], []]                   | 2.500     |
| 3.2   | [[1, 0, 0, 0, 0, 1], [[1, 3], [1, 3], [2, 4], [2, 4]], []]                 | 2.500     |
| 3.3   | [[1, 0, 0, 0, 0, 1], [[1, 3], [1, 4], [2, 3], [2, 4]], []]                 | 2.500     |
| 3.4   | [[1, 0, 0, 0, 0, 1], [[1, 2, 3, 4], [1, 2, 3, 4]], []]                     | 2.500     |
| 8.1   | [[1, 1, 0, 0, 1, 1], [[1, 2, 3, 4]], []]                                   | 3.000     |
| 8.2   | [[1, 1, 0, 0, 1, 1], [[1, 2, 3], [4]], []]                                 | 3.000     |
| 8.3   | [[1, 1, 0, 0, 1, 1], [[1, 2], [3], [4]], []]                               | 3.000     |
| 8.4   | [[1, 1, 0, 0, 1, 1], [[1, 4], [2], [3]], []]                               | 3.000     |
| 8.5   | [[1, 1, 0, 0, 1, 1], [[1], [2], [3], [4]], []]                             | 3.000     |
| 8.6   | [[1, 1, 0, 0, 1, 1], [[1, 2], [3, 4]], []]                                 | 3.000     |
| 8.7   | [[1, 1, 0, 0, 1, 1], [[1, 4], [2, 3]], []]                                 | 3.000     |
| 11.1  | [[1, 1, 1, 1, 1, 1], [], []]                                               | 3.500     |

## Acknowledgements

This research was supported via an LMS Undergraduate Research Bursary in 2018 for Leyna Watson May.

## References

- [CKLLS17] D. Cushing, R. Kangaslampi, V. Lipiäinen, Sh. Liu, G. W. Stagg, *The Graph Curvature Calculator and the curvatures of cubic graphs*, arXiv:1712.03033.
