# Supplementary material for: Quartic graphs which are Bakry-\'Emery curvature sharp
Source: arXiv:1902.10665 ancillary file (2019-02-27)
Supplement: Supplementary file 2 [file non_negative_classification.pdf]

# Incomplete 2-Balls with Non-negatively Curved Centre for Quartic Graphs

Francis Gurr and Leyna Watson May

## Abstract

This document contains the 204 incomplete 2-balls with non-negative curvature at their centres, separated by structure of the 1-ball. Additionally, it contains the 22 2-balls with infinity curvature sharp centres. This Latex document was generated by a Python program with the help of a curvature calculator written by David Cushing and George Stagg, see [CKLLS17].

## Representation of 2-balls

The (incomplete) 2-balls of quartic graphs listed in this article are represented in the following way. We fix a vertex  $v_0$  and  $S_1(v_0) = \{v_1, v_2, v_3, v_4\}$  (since in a quartic graph,  $v_0$  has four neighbors). The vertices of the 2-sphere are labeled as follows:  $S_2(v_0) = \{v_5, v_6, \dots, v_m\}$ . Then a 2-ball  $B_2(v_0)$  centered at  $v_0$  is represented by a list of 3 lists:  $B_2(v_0) = [list_1, list_2, list_3]$ . The first list determines the  $S_1$  structure (i.e., how the vertices in  $S_1$  are connected to each other) by  $list_1 = [a_{12}, a_{13}, a_{14}, a_{23}, a_{24}, a_{34}]$  where each  $a_{ij} \in \{0, 1\}$  is a Boolean indicator whether vertices  $v_i$  and  $v_j$  are adjacent or not. The second list  $list_2 = [a_5, a_6, \dots, a_m]$  describes the  $S_1$ - $S_2$  structure (i.e., which vertices in  $S_2$  are adjacent to vertices in  $S_1$ ). For instance,  $a_5 = [1, 2, 3]$  means that the vertex  $v_5$  is adjacent to  $v_1, v_2, v_3$  but not to  $v_4$ . Lastly, the list  $list_3$  describes the  $S_2$  structure (i.e., how the vertices in  $S_2$  are connected to each other). For example,  $list_3 = [[5, 7], [5, 8], [6, 8]]$  means that  $v_5 \sim v_7$ ,  $v_5 \sim v_8$ , and  $v_6 \sim v_8$ . However, the computation of Bakry-Émery curvature only requires the information of incomplete 2-balls where no spherical edge of  $S_2(v_0)$  is present, in which case  $list_3 = []$ .

The 11 1-ball structures and relevant properties are summarised in the following table:

| Index | 1-ball             | $S_1$ -out regular | upper Bakry-Émery curvature bound | Total number of non-negative 2-balls |
|-------|--------------------|--------------------|-----------------------------------|--------------------------------------|
| 1     | [0, 0, 0, 0, 0, 0] | True               | 2.000                             | 46                                   |
| 2     | [1, 0, 0, 0, 0, 0] | False              | 2.250                             | 55                                   |
| 3     | [1, 0, 0, 0, 0, 1] | True               | 2.500                             | 24                                   |
| 4     | [1, 1, 0, 0, 0, 0] | False              | 2.500                             | 31                                   |
| 5     | [1, 1, 1, 0, 0, 0] | False              | 2.750                             | 8                                    |
| 6     | [1, 1, 0, 1, 0, 0] | False              | 2.750                             | 4                                    |
| 7     | [1, 1, 0, 0, 1, 0] | False              | 2.750                             | 21                                   |
| 8     | [1, 1, 0, 0, 1, 1] | True               | 3.000                             | 7                                    |
| 9     | [1, 1, 1, 1, 0, 0] | False              | 3.000                             | 5                                    |
| 10    | [1, 1, 1, 1, 1, 0] | False              | 3.250                             | 2                                    |
| 11    | [1, 1, 1, 1, 1, 1] | True               | 3.500                             | 1                                    |

1  $list_1 = [0, 0, 0, 0, 0, 0]$

$S_1$ -out regular: True

Curvature bound: 2.000

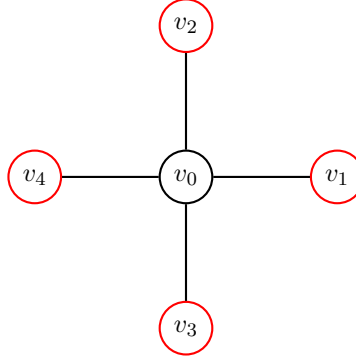

| Index | $[list_2, list_3]$                                           | Curvature | Curvature sharp |
|-------|--------------------------------------------------------------|-----------|-----------------|
| 1.1   | [[[1, 2, 3, 4], [1, 2, 3, 4], [1], [2], [3], [4]], []]       | 2.000     | True            |
| 1.2   | [[[1, 2, 3, 4], [1, 2, 3, 4], [1, 2], [3], [4]], []]         | 2.000     | True            |
| 1.3   | [[[1, 2, 3, 4], [1, 2, 3, 4], [1, 2, 3], [4]], []]           | 2.000     | True            |
| 1.4   | [[[1, 2, 3, 4], [1, 2], [1, 3], [2, 4], [3, 4]], []]         | 2.000     | True            |
| 1.5   | [[[1, 2], [1, 3], [1, 4], [2, 3], [2, 4], [3, 4]], []]       | 2.000     | True            |
| 1.6   | [[[1, 2, 3], [1, 2, 3], [1, 4], [2, 4], [3, 4]], []]         | 2.000     | True            |
| 1.7   | [[[1, 2, 3, 4], [1, 2, 3, 4], [1, 2], [3, 4]], []]           | 2.000     | True            |
| 1.8   | [[[1, 2, 3, 4], [1, 2, 3], [1, 2, 4], [3, 4]], []]           | 2.000     | True            |
| 1.9   | [[[1, 2, 3], [1, 2, 4], [1, 3, 4], [2, 3, 4]], []]           | 2.000     | True            |
| 1.10  | [[[1, 2, 3, 4], [1, 2, 3, 4], [1, 2, 3, 4]], []]             | 2.000     | True            |
| 1.11  | [[[1, 2, 3], [1, 2, 4], [1, 3], [2, 4], [3, 4]], []]         | 1.612     | False           |
| 1.12  | [[[1, 2, 3, 4], [1, 2, 3], [1, 4], [2, 4], [3]], []]         | 1.542     | False           |
| 1.13  | [[[1, 2, 3], [1, 2, 4], [1, 3, 4], [2], [3], [4]], []]       | 1.333     | False           |
| 1.14  | [[[1, 2, 3, 4], [1, 2, 3], [1, 2, 4], [3], [4]], []]         | 1.333     | False           |
| 1.15  | [[[1, 2, 3], [1, 2, 4], [1, 3, 4], [2, 3], [4]], []]         | 1.333     | False           |
| 1.16  | [[[1, 2, 3], [1, 2, 3], [1, 2, 4], [3, 4], [4]], []]         | 1.057     | False           |
| 1.17  | [[[1, 2, 3], [1, 4], [2, 4], [3, 4], [1], [2], [3]], []]     | 1.000     | False           |
| 1.18  | [[[1, 2, 3], [1, 2, 4], [1, 3], [3, 4], [2], [4]], []]       | 1.000     | False           |
| 1.19  | [[[1, 2, 3], [1, 2], [1, 4], [2, 4], [3, 4], [3]], []]       | 1.000     | False           |
| 1.20  | [[[1, 2, 3, 4], [1, 2, 3], [1, 4], [2], [3], [4]], []]       | 0.845     | False           |
| 1.21  | [[[1, 2, 3, 4], [1, 2, 3], [1, 2], [3, 4], [4]], []]         | 0.845     | False           |
| 1.22  | [[[1, 2, 3], [1, 2, 4], [3, 4], [1], [2], [3], [4]], []]     | 0.666     | False           |
| 1.23  | [[[1, 2, 3], [1, 2, 4], [1, 2], [3, 4], [3], [4]], []]       | 0.666     | False           |
| 1.24  | [[[1, 2, 3], [1, 2, 4], [3, 4], [3, 4], [1], [2]], []]       | 0.666     | False           |
| 1.25  | [[[1, 2, 3], [1, 2, 4], [1, 2], [3, 4], [3, 4]], []]         | 0.666     | False           |
| 1.26  | [[[1, 2, 3, 4], [1, 2], [1, 3], [2, 4], [3], [4]], []]       | 0.585     | False           |
| 1.27  | [[[1, 2, 3], [1, 2], [1, 3], [2, 4], [3, 4], [4]], []]       | 0.367     | False           |
| 1.28  | [[[1, 2, 3], [1, 2, 3], [1, 4], [2, 4], [3], [4]], []]       | 0.241     | False           |
| 1.29  | [[[1, 2, 3], [1, 2], [1, 4], [3, 4], [3, 4], [2]], []]       | 0.078     | False           |
| 1.30  | [[[1, 2, 3, 4], [1], [1], [2], [2], [3], [3], [4], [4]], []] | 0.000     | False           |
| 1.31  | [[[1, 2, 3, 4], [1, 2], [1], [2], [3], [3], [4], [4]], []]   | 0.000     | False           |
| 1.32  | [[[1, 2, 3, 4], [1, 2, 3], [1], [2], [3], [4], [4]], []]     | 0.000     | False           |

| Index | $[list_2, list_3]$                                           | Curvature | Curvature sharp |
|-------|--------------------------------------------------------------|-----------|-----------------|
| 1.33  | $[[[1, 2, 3, 4], [1, 2], [1, 2], [3], [3], [4], [4]], []]$   | 0.000     | False           |
| 1.34  | $[[[1, 2, 3, 4], [1, 2], [1, 3], [2], [3], [4], [4]], []]$   | 0.000     | False           |
| 1.35  | $[[[1, 2, 3, 4], [1, 2], [3, 4], [1], [2], [3], [4]], []]$   | 0.000     | False           |
| 1.36  | $[[[1, 2], [1, 3], [2, 4], [3, 4], [1], [2], [3], [4]], []]$ | 0.000     | False           |
| 1.37  | $[[[1, 2, 3], [1, 2], [1, 4], [3, 4], [2], [3], [4]], []]$   | 0.000     | False           |
| 1.38  | $[[[1, 2, 3, 4], [1, 2, 3], [1, 2], [3], [4], [4]], []]$     | 0.000     | False           |
| 1.39  | $[[[1, 2, 3, 4], [1, 2], [1, 2], [3, 4], [3], [4]], []]$     | 0.000     | False           |
| 1.40  | $[[[1, 2, 3, 4], [1, 2], [1, 3], [2, 3], [4], [4]], []]$     | 0.000     | False           |
| 1.41  | $[[[1, 2], [1, 2], [1, 3], [2, 4], [3, 4], [3], [4]], []]$   | 0.000     | False           |
| 1.42  | $[[[1, 2], [1, 3], [1, 4], [2, 3], [2, 4], [3], [4]], []]$   | 0.000     | False           |
| 1.43  | $[[[1, 2, 3], [1, 2, 4], [1, 3], [2, 4], [3], [4]], []]$     | 0.000     | False           |
| 1.44  | $[[[1, 2, 3, 4], [1, 2, 3], [1, 2, 3], [4], [4]], []]$       | 0.000     | False           |
| 1.45  | $[[[1, 2, 3, 4], [1, 2], [1, 2], [3, 4], [3, 4]], []]$       | 0.000     | False           |
| 1.46  | $[[[1, 2], [1, 2], [1, 3], [2, 4], [3, 4], [3, 4]], []]$     | 0.000     | False           |

**2**  $list_1 = [1, 0, 0, 0, 0, 0]$

$S_1$ -out regular: False

Curvature bound: 2.250

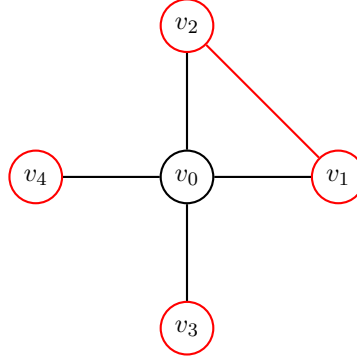

| Index | $[list_2, list_3]$                                 | Curvature | Curvature sharp |
|-------|----------------------------------------------------|-----------|-----------------|
| 2.1   | $[[[1, 3, 4], [2, 3, 4], [1, 3], [2, 4]], []]$     | 2.166     | False           |
| 2.2   | $[[[1, 2, 3, 4], [1, 3, 4], [2, 3, 4]], []]$       | 2.166     | False           |
| 2.3   | $[[[1, 3, 4], [1, 3, 4], [2, 3], [2, 4]], []]$     | 2.157     | False           |
| 2.4   | $[[[1, 2, 3, 4], [1, 2, 3, 4], [3], [4]], []]$     | 2.000     | False           |
| 2.5   | $[[[1, 2, 3, 4], [1, 3], [2, 4], [3, 4]], []]$     | 2.000     | False           |
| 2.6   | $[[[1, 3], [1, 4], [2, 3], [2, 4], [3, 4]], []]$   | 2.000     | False           |
| 2.7   | $[[[1, 2, 3, 4], [1, 2, 3, 4], [3, 4]], []]$       | 2.000     | False           |
| 2.8   | $[[[1, 3, 4], [1, 3, 4], [2, 3, 4], [2]], []]$     | 1.787     | False           |
| 2.9   | $[[[1, 2, 3], [1, 3, 4], [2, 4], [3, 4]], []]$     | 1.747     | False           |
| 2.10  | $[[[1, 2, 3, 4], [1, 3, 4], [2, 3], [4]], []]$     | 1.708     | False           |
| 2.11  | $[[[1, 2, 3], [1, 3, 4], [2, 3, 4], [4]], []]$     | 1.444     | False           |
| 2.12  | $[[[1, 3, 4], [2, 3], [2, 4], [3, 4], [1]], []]$   | 1.426     | False           |
| 2.13  | $[[[1, 3, 4], [2, 3, 4], [1, 3], [2], [4]], []]$   | 1.353     | False           |
| 2.14  | $[[[1, 2, 3, 4], [1, 3, 4], [2], [3], [4]], []]$   | 1.289     | False           |
| 2.15  | $[[[1, 2, 3, 4], [1, 3, 4], [3, 4], [2]], []]$     | 1.289     | False           |
| 2.16  | $[[[1, 3, 4], [1, 3], [2, 4], [3, 4], [2]], []]$   | 1.164     | False           |
| 2.17  | $[[[1, 2, 3], [1, 4], [2, 4], [3, 4], [3]], []]$   | 1.120     | False           |
| 2.18  | $[[[1, 3, 4], [1, 3], [2, 3], [2, 4], [4]], []]$   | 1.106     | False           |
| 2.19  | $[[[1, 2, 3], [1, 3, 4], [2, 4], [3], [4]], []]$   | 1.056     | False           |
| 2.20  | $[[[1, 3, 4], [2, 3], [2, 4], [1], [3], [4]], []]$ | 1.000     | False           |
| 2.21  | $[[[1, 2, 3, 4], [1, 2, 3], [3, 4], [4]], []]$     | 1.000     | False           |
| 2.22  | $[[[1, 3, 4], [1, 3, 4], [2, 3], [2], [4]], []]$   | 0.938     | False           |
| 2.23  | $[[[1, 3], [1, 3], [2, 4], [2, 4], [3, 4]], []]$   | 0.891     | False           |
| 2.24  | $[[[1, 3, 4], [2, 3, 4], [1], [2], [3], [4]], []]$ | 0.871     | False           |
| 2.25  | $[[[1, 2, 3], [1, 2, 4], [3, 4], [3], [4]], []]$   | 0.871     | False           |
| 2.26  | $[[[1, 3, 4], [2, 3, 4], [1, 2], [3], [4]], []]$   | 0.871     | False           |
| 2.27  | $[[[1, 3, 4], [2, 3, 4], [3, 4], [1], [2]], []]$   | 0.871     | False           |
| 2.28  | $[[[1, 2, 3], [1, 2, 4], [3, 4], [3, 4]], []]$     | 0.871     | False           |
| 2.29  | $[[[1, 3, 4], [2, 3, 4], [1, 2], [3, 4]], []]$     | 0.871     | False           |
| 2.30  | $[[[1, 2, 3, 4], [1, 3], [3, 4], [2], [4]], []]$   | 0.842     | False           |
| 2.31  | $[[[1, 2, 3, 4], [1, 3], [2, 4], [3], [4]], []]$   | 0.787     | False           |
| 2.32  | $[[[1, 3, 4], [1, 3], [2, 4], [2, 4], [3]], []]$   | 0.615     | False           |

| Index | $[list_2, list_3]$                                   | Curvature | Curvature sharp |
|-------|------------------------------------------------------|-----------|-----------------|
| 2.33  | $[[[1, 3, 4], [1, 3], [2, 4], [2], [3], [4]], []]$   | 0.614     | False           |
| 2.34  | $[[[1, 2, 3], [1, 3], [2, 4], [3, 4], [4]], []]$     | 0.561     | False           |
| 2.35  | $[[[1, 3], [1, 3], [2, 4], [3, 4], [2], [4]], []]$   | 0.543     | False           |
| 2.36  | $[[[1, 3], [1, 4], [2, 3], [3, 4], [2], [4]], []]$   | 0.427     | False           |
| 2.37  | $[[[1, 2, 3], [1, 4], [3, 4], [3, 4], [2]], []]$     | 0.404     | False           |
| 2.38  | $[[[1, 2, 3], [1, 4], [3, 4], [2], [3], [4]], []]$   | 0.321     | False           |
| 2.39  | $[[[1, 2, 3], [1, 3, 4], [3, 4], [2], [4]], []]$     | 0.321     | False           |
| 2.40  | $[[[1, 3, 4], [1, 2], [2, 3], [3, 4], [4]], []]$     | 0.294     | False           |
| 2.41  | $[[[1, 3, 4], [2, 3], [3, 4], [1], [2], [4]], []]$   | 0.278     | False           |
| 2.42  | $[[[1, 2, 3, 4], [3, 4], [1], [2], [3], [4]], []]$   | 0.219     | False           |
| 2.43  | $[[[1, 3], [2, 4], [3, 4], [1], [2], [3], [4]], []]$ | 0.219     | False           |
| 2.44  | $[[[1, 2, 3, 4], [1, 2], [3, 4], [3], [4]], []]$     | 0.219     | False           |
| 2.45  | $[[[1, 2, 3, 4], [3, 4], [3, 4], [1], [2]], []]$     | 0.219     | False           |
| 2.46  | $[[[1, 2], [1, 3], [2, 4], [3, 4], [3], [4]], []]$   | 0.219     | False           |
| 2.47  | $[[[1, 3], [2, 4], [3, 4], [3, 4], [1], [2]], []]$   | 0.219     | False           |
| 2.48  | $[[[1, 2, 3, 4], [1, 2], [3, 4], [3, 4]], []]$       | 0.219     | False           |
| 2.49  | $[[[1, 2], [1, 3], [2, 4], [3, 4], [3, 4]], []]$     | 0.219     | False           |
| 2.50  | $[[[1, 2, 3, 4], [1, 3], [2, 3], [4], [4]], []]$     | 0.070     | False           |
| 2.51  | $[[[1, 2, 3, 4], [1, 2, 3], [3], [4], [4]], []]$     | 0.068     | False           |
| 2.52  | $[[[1, 2, 3, 4], [1, 3], [2], [3], [4], [4]], []]$   | 0.066     | False           |
| 2.53  | $[[[1, 2, 3, 4], [1], [2], [3], [3], [4], [4]], []]$ | 0.000     | False           |
| 2.54  | $[[[1, 2, 3, 4], [1, 2], [3], [3], [4], [4]], []]$   | 0.000     | False           |
| 2.55  | $[[[1, 3], [1, 4], [2, 3], [2, 4], [3], [4]], []]$   | 0.000     | False           |

**3**  $list_1 = [1, 0, 0, 0, 0, 1]$

$S_1$ -out regular: True

Curvature bound: 2.500

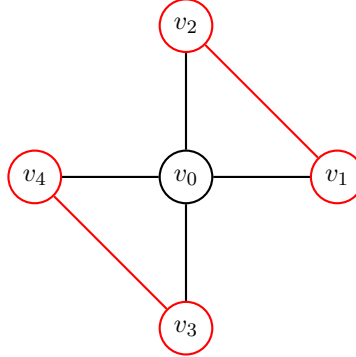

| Index | $[list_2, list_3]$                           | Curvature | Curvature sharp |
|-------|----------------------------------------------|-----------|-----------------|
| 3.1   | $[[[1, 2, 3, 4], [1, 3], [2, 4]], []]$       | 2.500     | True            |
| 3.2   | $[[[1, 3], [1, 3], [2, 4], [2, 4]], []]$     | 2.500     | True            |
| 3.3   | $[[[1, 3], [1, 4], [2, 3], [2, 4]], []]$     | 2.500     | True            |
| 3.4   | $[[[1, 2, 3, 4], [1, 2, 3, 4]], []]$         | 2.500     | True            |
| 3.5   | $[[[1, 2, 3], [1, 3, 4], [2, 4]], []]$       | 2.139     | False           |
| 3.6   | $[[[1, 2, 3], [1, 4], [2, 4], [3]], []]$     | 1.741     | False           |
| 3.7   | $[[[1, 2, 3, 4], [1, 2, 3], [4]], []]$       | 1.585     | False           |
| 3.8   | $[[[1, 2, 3], [1, 3], [2, 4], [4]], []]$     | 1.470     | False           |
| 3.9   | $[[[1, 2, 3, 4], [1, 3], [2], [4]], []]$     | 1.263     | False           |
| 3.10  | $[[[1, 3], [1, 3], [2, 4], [2], [4]], []]$   | 1.263     | False           |
| 3.11  | $[[[1, 2, 3], [1, 2, 4], [3], [4]], []]$     | 1.166     | False           |
| 3.12  | $[[[1, 2, 3], [1, 2, 4], [3, 4]], []]$       | 1.166     | False           |
| 3.13  | $[[[1, 3], [1, 4], [2, 3], [2], [4]], []]$   | 1.085     | False           |
| 3.14  | $[[[1, 2, 3], [1, 3, 4], [2], [4]], []]$     | 0.762     | False           |
| 3.15  | $[[[1, 2, 3], [1, 4], [3, 4], [2]], []]$     | 0.696     | False           |
| 3.16  | $[[[1, 2, 3], [1, 4], [2], [3], [4]], []]$   | 0.683     | False           |
| 3.17  | $[[[1, 2, 3, 4], [1], [2], [3], [4]], []]$   | 0.500     | False           |
| 3.18  | $[[[1, 3], [2, 4], [1], [2], [3], [4]], []]$ | 0.500     | False           |
| 3.19  | $[[[1, 2, 3, 4], [1, 2], [3], [4]], []]$     | 0.500     | False           |
| 3.20  | $[[[1, 2], [1, 3], [2, 4], [3], [4]], []]$   | 0.500     | False           |
| 3.21  | $[[[1, 2, 3, 4], [1, 2], [3, 4]], []]$       | 0.500     | False           |
| 3.22  | $[[[1, 2], [1, 3], [2, 4], [3, 4]], []]$     | 0.500     | False           |
| 3.23  | $[[[1, 2, 3], [1, 2, 3], [4], [4]], []]$     | 0.190     | False           |
| 3.24  | $[[[1, 2, 3], [1, 3], [2], [4], [4]], []]$   | 0.036     | False           |

4  $list_1 = [1, 1, 0, 0, 0, 0]$

$S_1$ -out regular: False

Curvature bound: 2.500

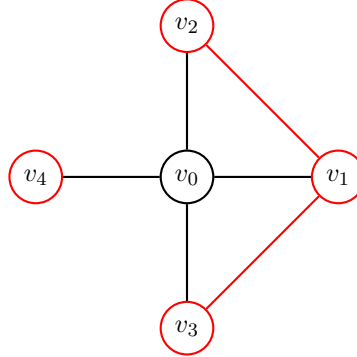

| Index | $[list_2, list_3]$                           | Curvature | Curvature sharp |
|-------|----------------------------------------------|-----------|-----------------|
| 4.1   | $[[[2, 3, 4], [2, 3, 4], [1, 4]], []]$       | 2.357     | False           |
| 4.2   | $[[[1, 2, 4], [2, 3, 4], [3, 4]], []]$       | 2.302     | False           |
| 4.3   | $[[[1, 2, 3, 4], [2, 4], [3, 4]], []]$       | 2.254     | False           |
| 4.4   | $[[[1, 4], [2, 3], [2, 4], [3, 4]], []]$     | 2.000     | False           |
| 4.5   | $[[[2, 3, 4], [1, 4], [2, 4], [3]], []]$     | 1.879     | False           |
| 4.6   | $[[[2, 3, 4], [2, 4], [3, 4], [1]], []]$     | 1.814     | False           |
| 4.7   | $[[[1, 2, 3, 4], [2, 3, 4], [4]], []]$       | 1.764     | False           |
| 4.8   | $[[[1, 2, 4], [2, 4], [3, 4], [3]], []]$     | 1.746     | False           |
| 4.9   | $[[[1, 4], [2, 4], [3, 4], [2], [3]], []]$   | 1.500     | False           |
| 4.10  | $[[[1, 2, 4], [2, 3, 4], [3], [4]], []]$     | 1.467     | False           |
| 4.11  | $[[[2, 3, 4], [2, 3, 4], [1], [4]], []]$     | 1.295     | False           |
| 4.12  | $[[[1, 2, 4], [3, 4], [3, 4], [2]], []]$     | 1.204     | False           |
| 4.13  | $[[[2, 3, 4], [1, 4], [2], [3], [4]], []]$   | 1.181     | False           |
| 4.14  | $[[[1, 2, 4], [2, 3], [3, 4], [4]], []]$     | 1.181     | False           |
| 4.15  | $[[[2, 3, 4], [1, 4], [2, 3], [4]], []]$     | 1.181     | False           |
| 4.16  | $[[[1, 2], [2, 4], [3, 4], [3, 4]], []]$     | 1.110     | False           |
| 4.17  | $[[[2, 4], [2, 4], [3, 4], [1], [3]], []]$   | 1.091     | False           |
| 4.18  | $[[[1, 2, 3, 4], [2, 4], [3], [4]], []]$     | 1.081     | False           |
| 4.19  | $[[[1, 2, 4], [3, 4], [2], [3], [4]], []]$   | 1.075     | False           |
| 4.20  | $[[[2, 3, 4], [2, 4], [1], [3], [4]], []]$   | 0.746     | False           |
| 4.21  | $[[[2, 3, 4], [1, 2], [3, 4], [4]], []]$     | 0.746     | False           |
| 4.22  | $[[[1, 2, 3], [2, 4], [3, 4], [4]], []]$     | 0.674     | False           |
| 4.23  | $[[[1, 2], [2, 4], [3, 4], [3], [4]], []]$   | 0.653     | False           |
| 4.24  | $[[[2, 4], [3, 4], [1], [2], [3], [4]], []]$ | 0.626     | False           |
| 4.25  | $[[[2, 3], [2, 4], [3, 4], [1], [4]], []]$   | 0.626     | False           |
| 4.26  | $[[[1, 4], [2, 3], [2, 4], [3], [4]], []]$   | 0.448     | False           |
| 4.27  | $[[[1, 2, 3, 4], [2], [3], [4], [4]], []]$   | 0.130     | False           |
| 4.28  | $[[[1, 2, 3, 4], [2, 3], [4], [4]], []]$     | 0.130     | False           |
| 4.29  | $[[[1, 4], [2, 4], [2, 4], [3], [3]], []]$   | 0.107     | False           |
| 4.30  | $[[[1, 2, 4], [2, 4], [3], [3], [4]], []]$   | 0.012     | False           |
| 4.31  | $[[[1, 4], [2, 4], [2], [3], [3], [4]], []]$ | 0.010     | False           |

5  $list_1 = [1, 1, 1, 0, 0, 0]$

$S_1$ -out regular: False

Curvature bound: 2.750

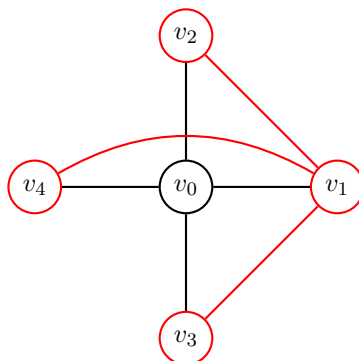

| Index | $[list_2, list_3]$                     | Curvature | Curvature sharp |
|-------|----------------------------------------|-----------|-----------------|
| 5.1   | $[[[2, 3], [2, 4], [3, 4]], []]$       | 2.708     | False           |
| 5.2   | $[[[2, 3, 4], [2, 3, 4]], []]$         | 2.708     | False           |
| 5.3   | $[[[2, 3, 4], [2], [3], [4]], []]$     | 2.500     | False           |
| 5.4   | $[[[2, 3, 4], [2, 3], [4]], []]$       | 2.500     | False           |
| 5.5   | $[[[2, 3], [2, 4], [3], [4]], []]$     | 1.500     | False           |
| 5.6   | $[[[2, 3], [2], [3], [4], [4]], []]$   | 0.500     | False           |
| 5.7   | $[[[2], [2], [3], [3], [4], [4]], []]$ | 0.500     | False           |
| 5.8   | $[[[2, 3], [2, 3], [4], [4]], []]$     | 0.500     | False           |



**6**  $list_1 = [1, 1, 0, 1, 0, 0]$

$S_1$ -out regular: False

Curvature bound: 2.750

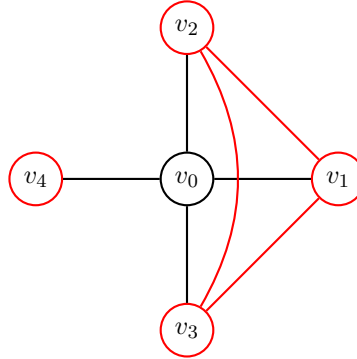

| Index | $[list_2, list_3]$                 | Curvature | Curvature sharp |
|-------|------------------------------------|-----------|-----------------|
| 6.1   | $[[[1, 4], [2, 4], [3, 4]], []]$   | 2.000     | False           |
| 6.2   | $[[[1, 2, 4], [3, 4], [4]], []]$   | 1.217     | False           |
| 6.3   | $[[[1, 4], [2, 4], [3], [4]], []]$ | 0.638     | False           |
| 6.4   | $[[[1, 2, 3, 4], [4], [4]], []]$   | 0.177     | False           |

**7**  $list_1 = [1, 1, 0, 0, 1, 0]$

$S_1$ -out regular: False

Curvature bound: 2.750

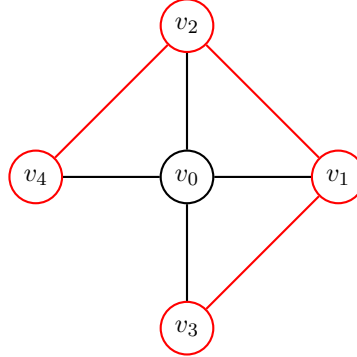

| Index | $[list_2, list_3]$                 | Curvature | Curvature sharp |
|-------|------------------------------------|-----------|-----------------|
| 7.1   | [[[1, 3, 4], [2, 3, 4]], []]       | 2.726     | False           |
| 7.2   | [[[1, 2, 3, 4], [3, 4]], []]       | 2.719     | False           |
| 7.3   | [[[1, 4], [2, 3], [3, 4]], []]     | 2.719     | False           |
| 7.4   | [[[1, 3, 4], [3, 4], [2]], []]     | 2.622     | False           |
| 7.5   | [[[3, 4], [3, 4], [1], [2]], []]   | 2.500     | False           |
| 7.6   | [[[1, 2], [3, 4], [3, 4]], []]     | 2.500     | False           |
| 7.7   | [[[1, 3, 4], [2, 3], [4]], []]     | 2.278     | False           |
| 7.8   | [[[1, 2, 3], [3, 4], [4]], []]     | 1.944     | False           |
| 7.9   | [[[1, 4], [3, 4], [2], [3]], []]   | 1.816     | False           |
| 7.10  | [[[1, 2, 3, 4], [3], [4]], []]     | 1.739     | False           |
| 7.11  | [[[1, 2], [3, 4], [3], [4]], []]   | 1.739     | False           |
| 7.12  | [[[1, 3], [2, 4], [3, 4]], []]     | 1.500     | False           |
| 7.13  | [[[1, 3, 4], [2, 4], [3]], []]     | 1.473     | False           |
| 7.14  | [[[1, 3, 4], [2], [3], [4]], []]   | 1.463     | False           |
| 7.15  | [[[1, 3], [3, 4], [2], [4]], []]   | 1.429     | False           |
| 7.16  | [[[3, 4], [1], [2], [3], [4]], []] | 1.391     | False           |
| 7.17  | [[[1, 4], [2, 3], [3], [4]], []]   | 1.287     | False           |
| 7.18  | [[[1, 3], [2, 3], [4], [4]], []]   | 0.337     | False           |
| 7.19  | [[[1, 2, 3], [3], [4], [4]], []]   | 0.328     | False           |
| 7.20  | [[[1, 4], [2], [3], [3], [4]], []] | 0.315     | False           |
| 7.21  | [[[1, 3], [2, 4], [3], [4]], []]   | 0.000     | False           |

8  $list_1 = [1, 1, 0, 0, 1, 1]$

$S_1$ -out regular: True

Curvature bound: 3.000

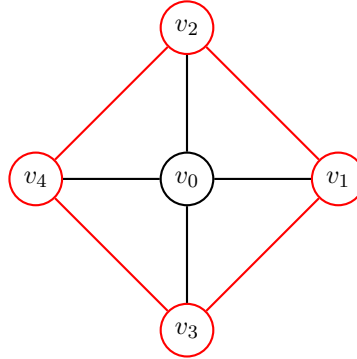

| Index | $[list_2, list_3]$           | Curvature | Curvature sharp |
|-------|------------------------------|-----------|-----------------|
| 8.1   | $[[[1, 2, 3, 4]], []]$       | 3.000     | True            |
| 8.2   | $[[[1, 2, 3], [4]], []]$     | 3.000     | True            |
| 8.3   | $[[[1, 2], [3], [4]], []]$   | 3.000     | True            |
| 8.4   | $[[[1, 4], [2], [3]], []]$   | 3.000     | True            |
| 8.5   | $[[[1], [2], [3], [4]], []]$ | 3.000     | True            |
| 8.6   | $[[[1, 2], [3, 4]], []]$     | 3.000     | True            |
| 8.7   | $[[[1, 4], [2, 3]], []]$     | 3.000     | True            |

**9**  $list_1 = [1, 1, 1, 1, 0, 0]$

$S_1$ -out regular: False

Curvature bound: 3.000

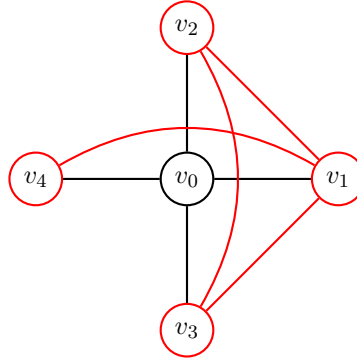

| Index | $[list_2, list_3]$           | Curvature | Curvature sharp |
|-------|------------------------------|-----------|-----------------|
| 9.1   | $[[[2, 4], [3, 4]], []]$     | 2.920     | False           |
| 9.2   | $[[[2, 3, 4], [4]], []]$     | 2.558     | False           |
| 9.3   | $[[[2, 4], [3], [4]], []]$   | 1.913     | False           |
| 9.4   | $[[[2, 3], [4], [4]], []]$   | 0.645     | False           |
| 9.5   | $[[[2], [3], [4], [4]], []]$ | 0.645     | False           |

**10**  $list_1 = [1, 1, 1, 1, 1, 0]$

$S_1$ -out regular: False

Curvature bound: 3.250

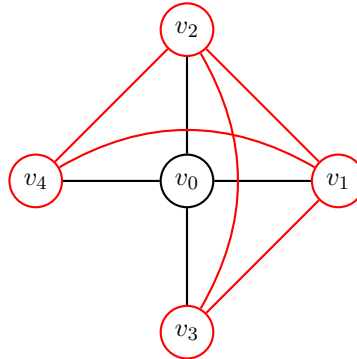

| Index | $[list_2, list_3]$ | Curvature | Curvature sharp |
|-------|--------------------|-----------|-----------------|
| 10.1  | $[[[3, 4]], []]$   | 3.234     | False           |
| 10.2  | $[[[3], [4]], []]$ | 3.000     | False           |

**11**     $list_1 = [1, 1, 1, 1, 1, 1]$

$S_1$ -out regular: True

Curvature bound: 3.500

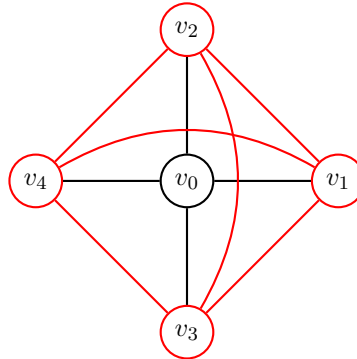

| Index | $[list_2, list_3]$   | Curvature | Curvature sharp |
|-------|----------------------|-----------|-----------------|
| 11.1  | $[\square, \square]$ | 3.500     | True            |

## Curvature Sharp Graphs

Total: 22

| Index | Incomplete 2-ball                                                          | Curvature |
|-------|----------------------------------------------------------------------------|-----------|
| 1.1   | [[0, 0, 0, 0, 0, 0], [[1, 2, 3, 4], [1, 2, 3, 4], [1], [2], [3], [4]], []] | 2.000     |
| 1.2   | [[0, 0, 0, 0, 0, 0], [[1, 2, 3, 4], [1, 2, 3, 4], [1, 2], [3], [4]], []]   | 2.000     |
| 1.3   | [[0, 0, 0, 0, 0, 0], [[1, 2, 3, 4], [1, 2, 3, 4], [1, 2, 3], [4]], []]     | 2.000     |
| 1.4   | [[0, 0, 0, 0, 0, 0], [[1, 2, 3, 4], [1, 2], [1, 3], [2, 4], [3, 4]], []]   | 2.000     |
| 1.5   | [[0, 0, 0, 0, 0, 0], [[1, 2], [1, 3], [1, 4], [2, 3], [2, 4], [3, 4]], []] | 2.000     |
| 1.6   | [[0, 0, 0, 0, 0, 0], [[1, 2, 3], [1, 2, 3], [1, 4], [2, 4], [3, 4]], []]   | 2.000     |
| 1.7   | [[0, 0, 0, 0, 0, 0], [[1, 2, 3, 4], [1, 2, 3, 4], [1, 2], [3, 4]], []]     | 2.000     |
| 1.8   | [[0, 0, 0, 0, 0, 0], [[1, 2, 3, 4], [1, 2, 3], [1, 2, 4], [3, 4]], []]     | 2.000     |
| 1.9   | [[0, 0, 0, 0, 0, 0], [[1, 2, 3], [1, 2, 4], [1, 3, 4], [2, 3, 4]], []]     | 2.000     |
| 1.10  | [[0, 0, 0, 0, 0, 0], [[1, 2, 3, 4], [1, 2, 3, 4], [1, 2, 3, 4]], []]       | 2.000     |
| 3.1   | [[1, 0, 0, 0, 0, 1], [[1, 2, 3, 4], [1, 3], [2, 4]], []]                   | 2.500     |
| 3.2   | [[1, 0, 0, 0, 0, 1], [[1, 3], [1, 3], [2, 4], [2, 4]], []]                 | 2.500     |
| 3.3   | [[1, 0, 0, 0, 0, 1], [[1, 3], [1, 4], [2, 3], [2, 4]], []]                 | 2.500     |
| 3.4   | [[1, 0, 0, 0, 0, 1], [[1, 2, 3, 4], [1, 2, 3, 4]], []]                     | 2.500     |
| 8.1   | [[1, 1, 0, 0, 1, 1], [[1, 2, 3, 4]], []]                                   | 3.000     |
| 8.2   | [[1, 1, 0, 0, 1, 1], [[1, 2, 3], [4]], []]                                 | 3.000     |
| 8.3   | [[1, 1, 0, 0, 1, 1], [[1, 2], [3], [4]], []]                               | 3.000     |
| 8.4   | [[1, 1, 0, 0, 1, 1], [[1, 4], [2], [3]], []]                               | 3.000     |
| 8.5   | [[1, 1, 0, 0, 1, 1], [[1], [2], [3], [4]], []]                             | 3.000     |
| 8.6   | [[1, 1, 0, 0, 1, 1], [[1, 2], [3, 4]], []]                                 | 3.000     |
| 8.7   | [[1, 1, 0, 0, 1, 1], [[1, 4], [2, 3]], []]                                 | 3.000     |
| 11.1  | [[1, 1, 1, 1, 1, 1], [], []]                                               | 3.500     |

## Acknowledgements

This research was supported via an LMS Undergraduate Research Bursary in 2018 for Leyna Watson May.

## References

- [CKLLS17] D. Cushing, R. Kangaslampi, V. Lipiäinen, Sh. Liu, G. W. Stagg, *The Graph Curvature Calculator and the curvatures of cubic graphs*, arXiv:1712.03033.
